# Supplementary material for: The Shortest Route Is Not Always the Fastest: Probability-Modeled Stereoscopic Eye Movement Completion Time in VR
Source: arXiv:2309.15183 source file (2023-10-03)
Supplement: Supplementary file 1 [file fig_supp_ablation_histograms.tex]

\begin{figure}[h]
    \centering
    \subfloat[$\conditionAccuracySaccade$, divergent]{
        \includegraphics[width=0.47\linewidth]{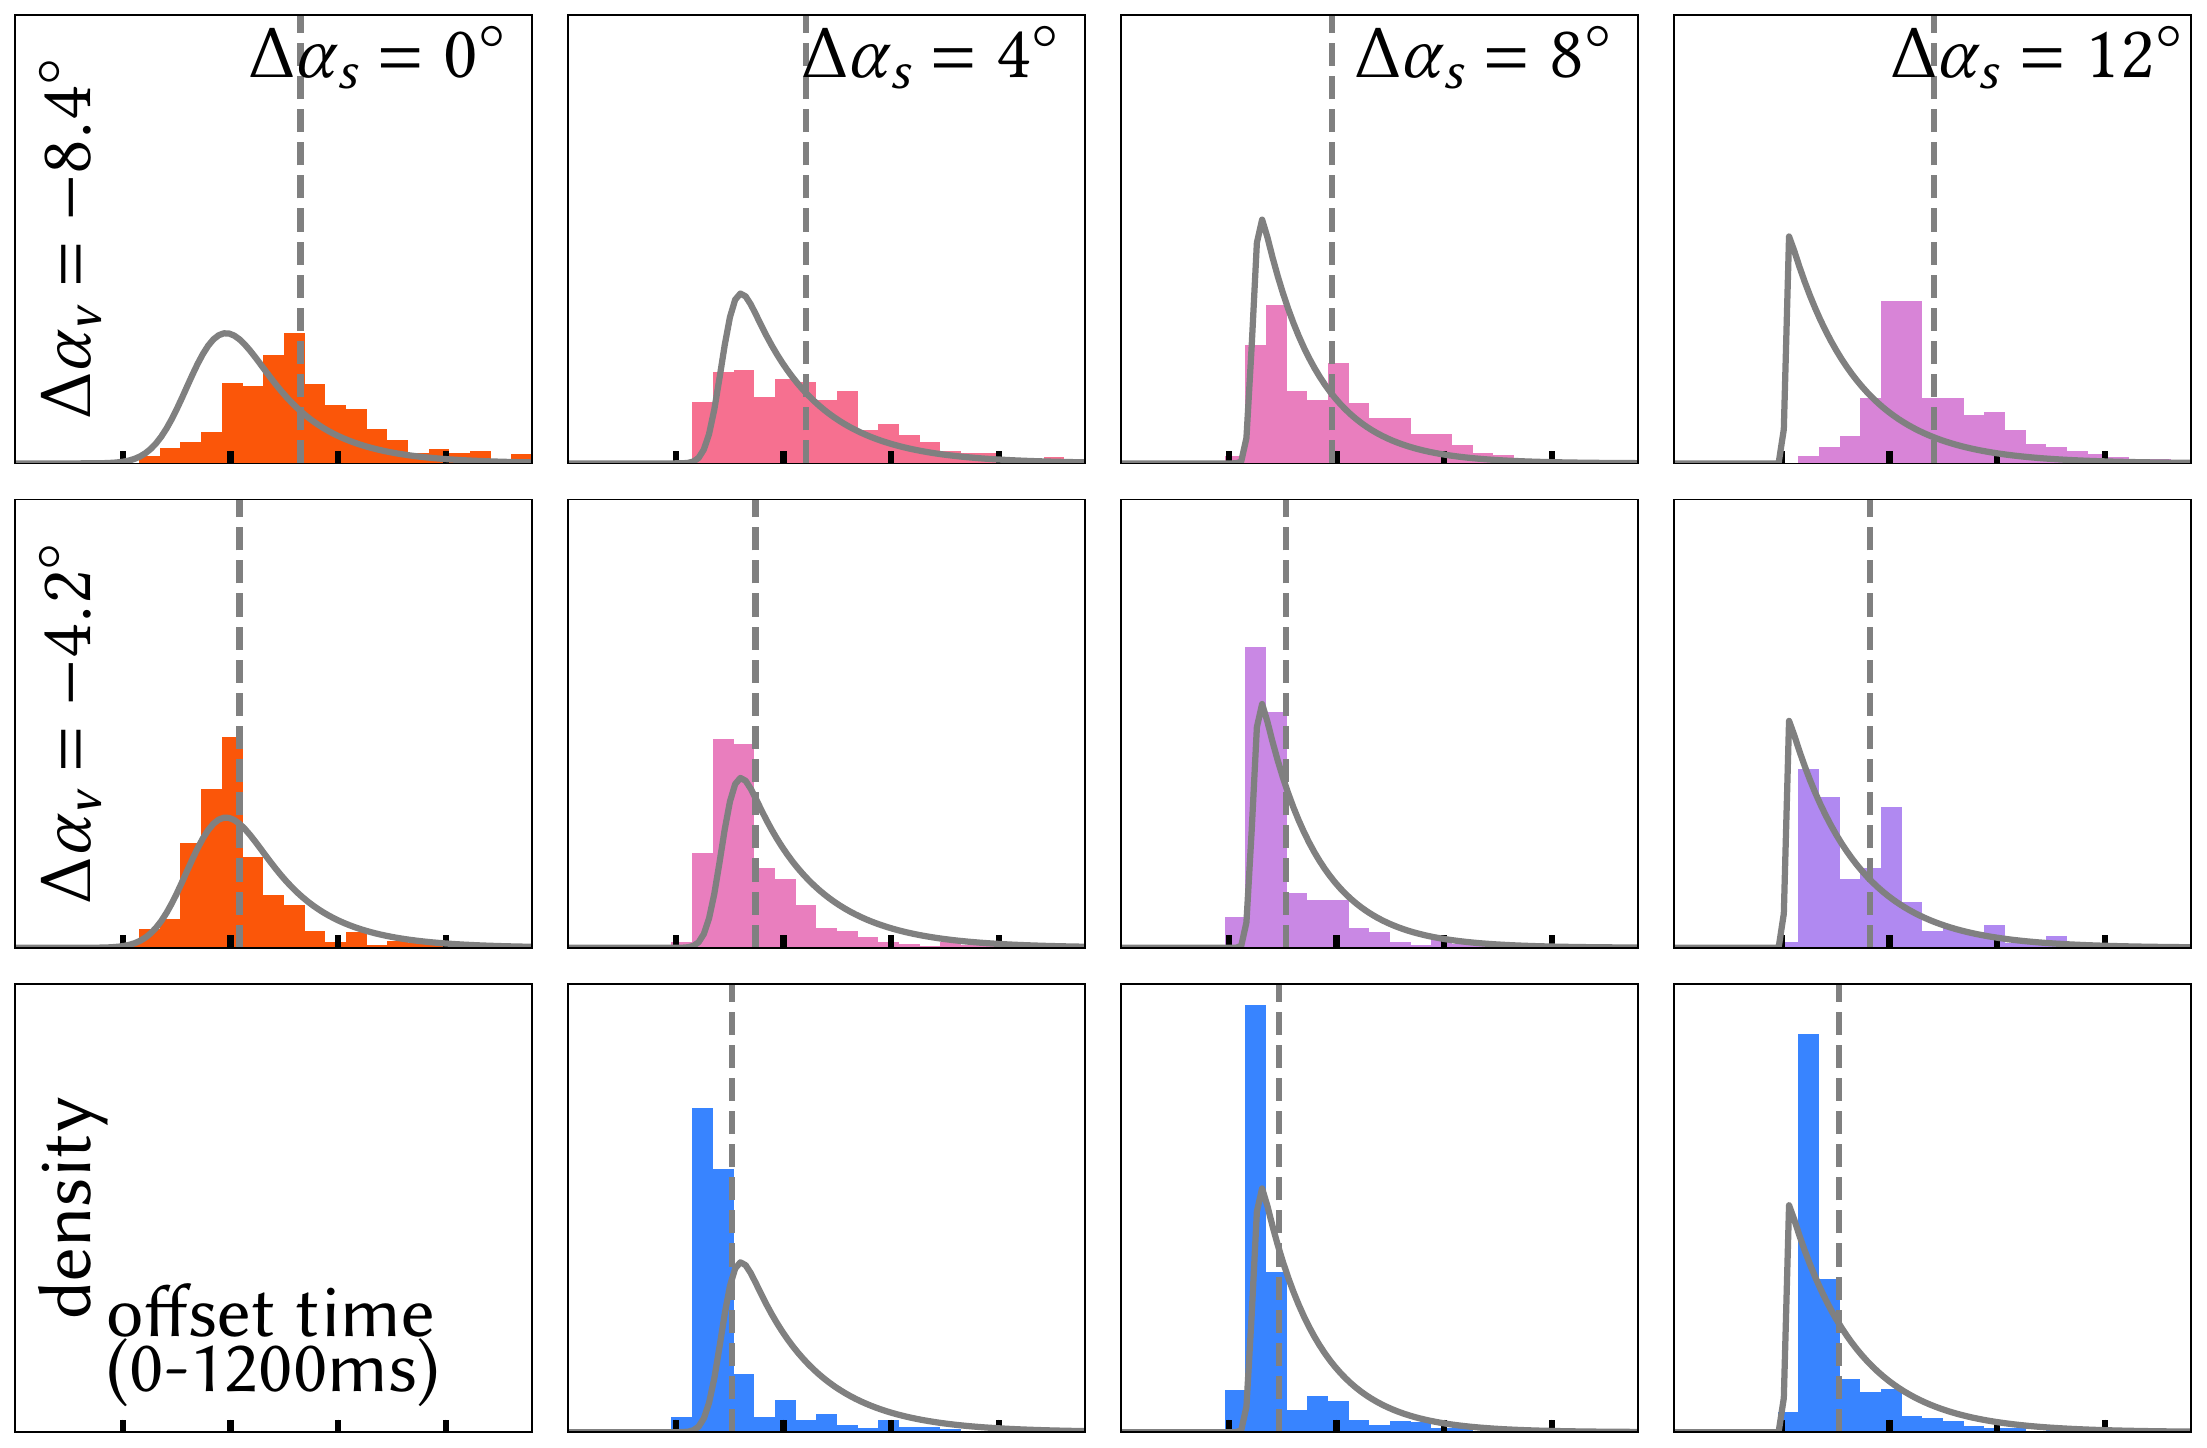}
        \label{fig:supp:ablation:saccade:div}
    }%subfloat
    \subfloat[$\conditionAccuracySaccade$, convergent]{
        \includegraphics[width=0.47\linewidth]{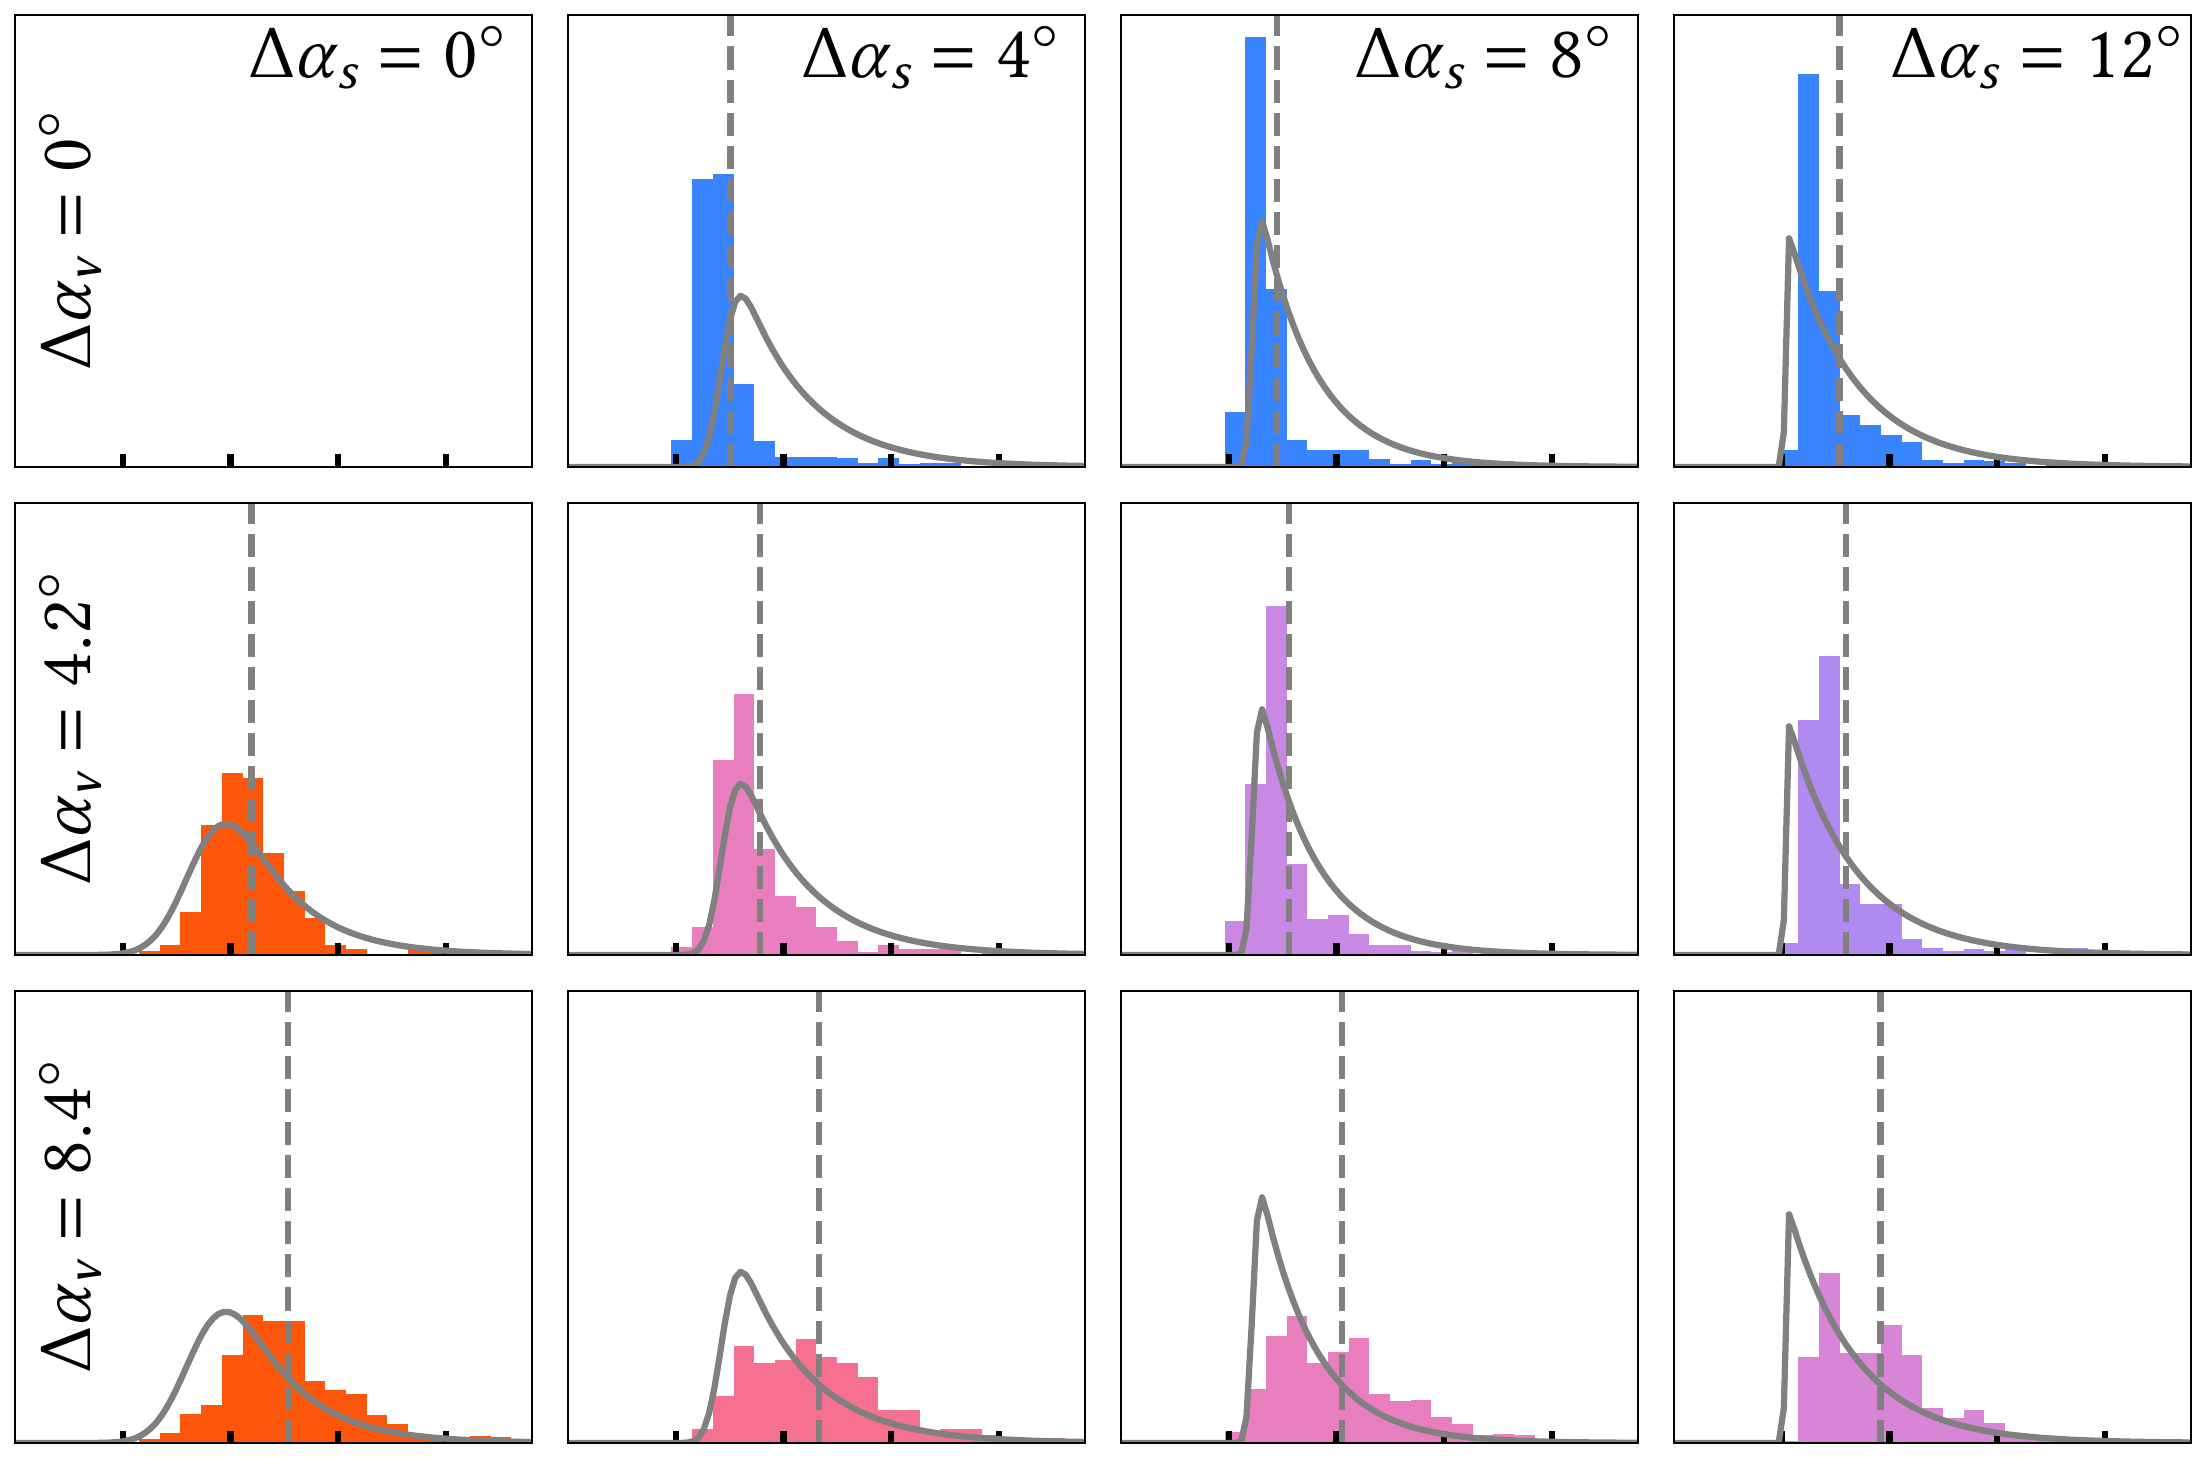}
        \label{fig:supp:ablation:saccade:con}
    }%subfloat
    
    \subfloat[$\conditionAccuracyVergence$, divergent]{
        \includegraphics[width=0.47\linewidth]{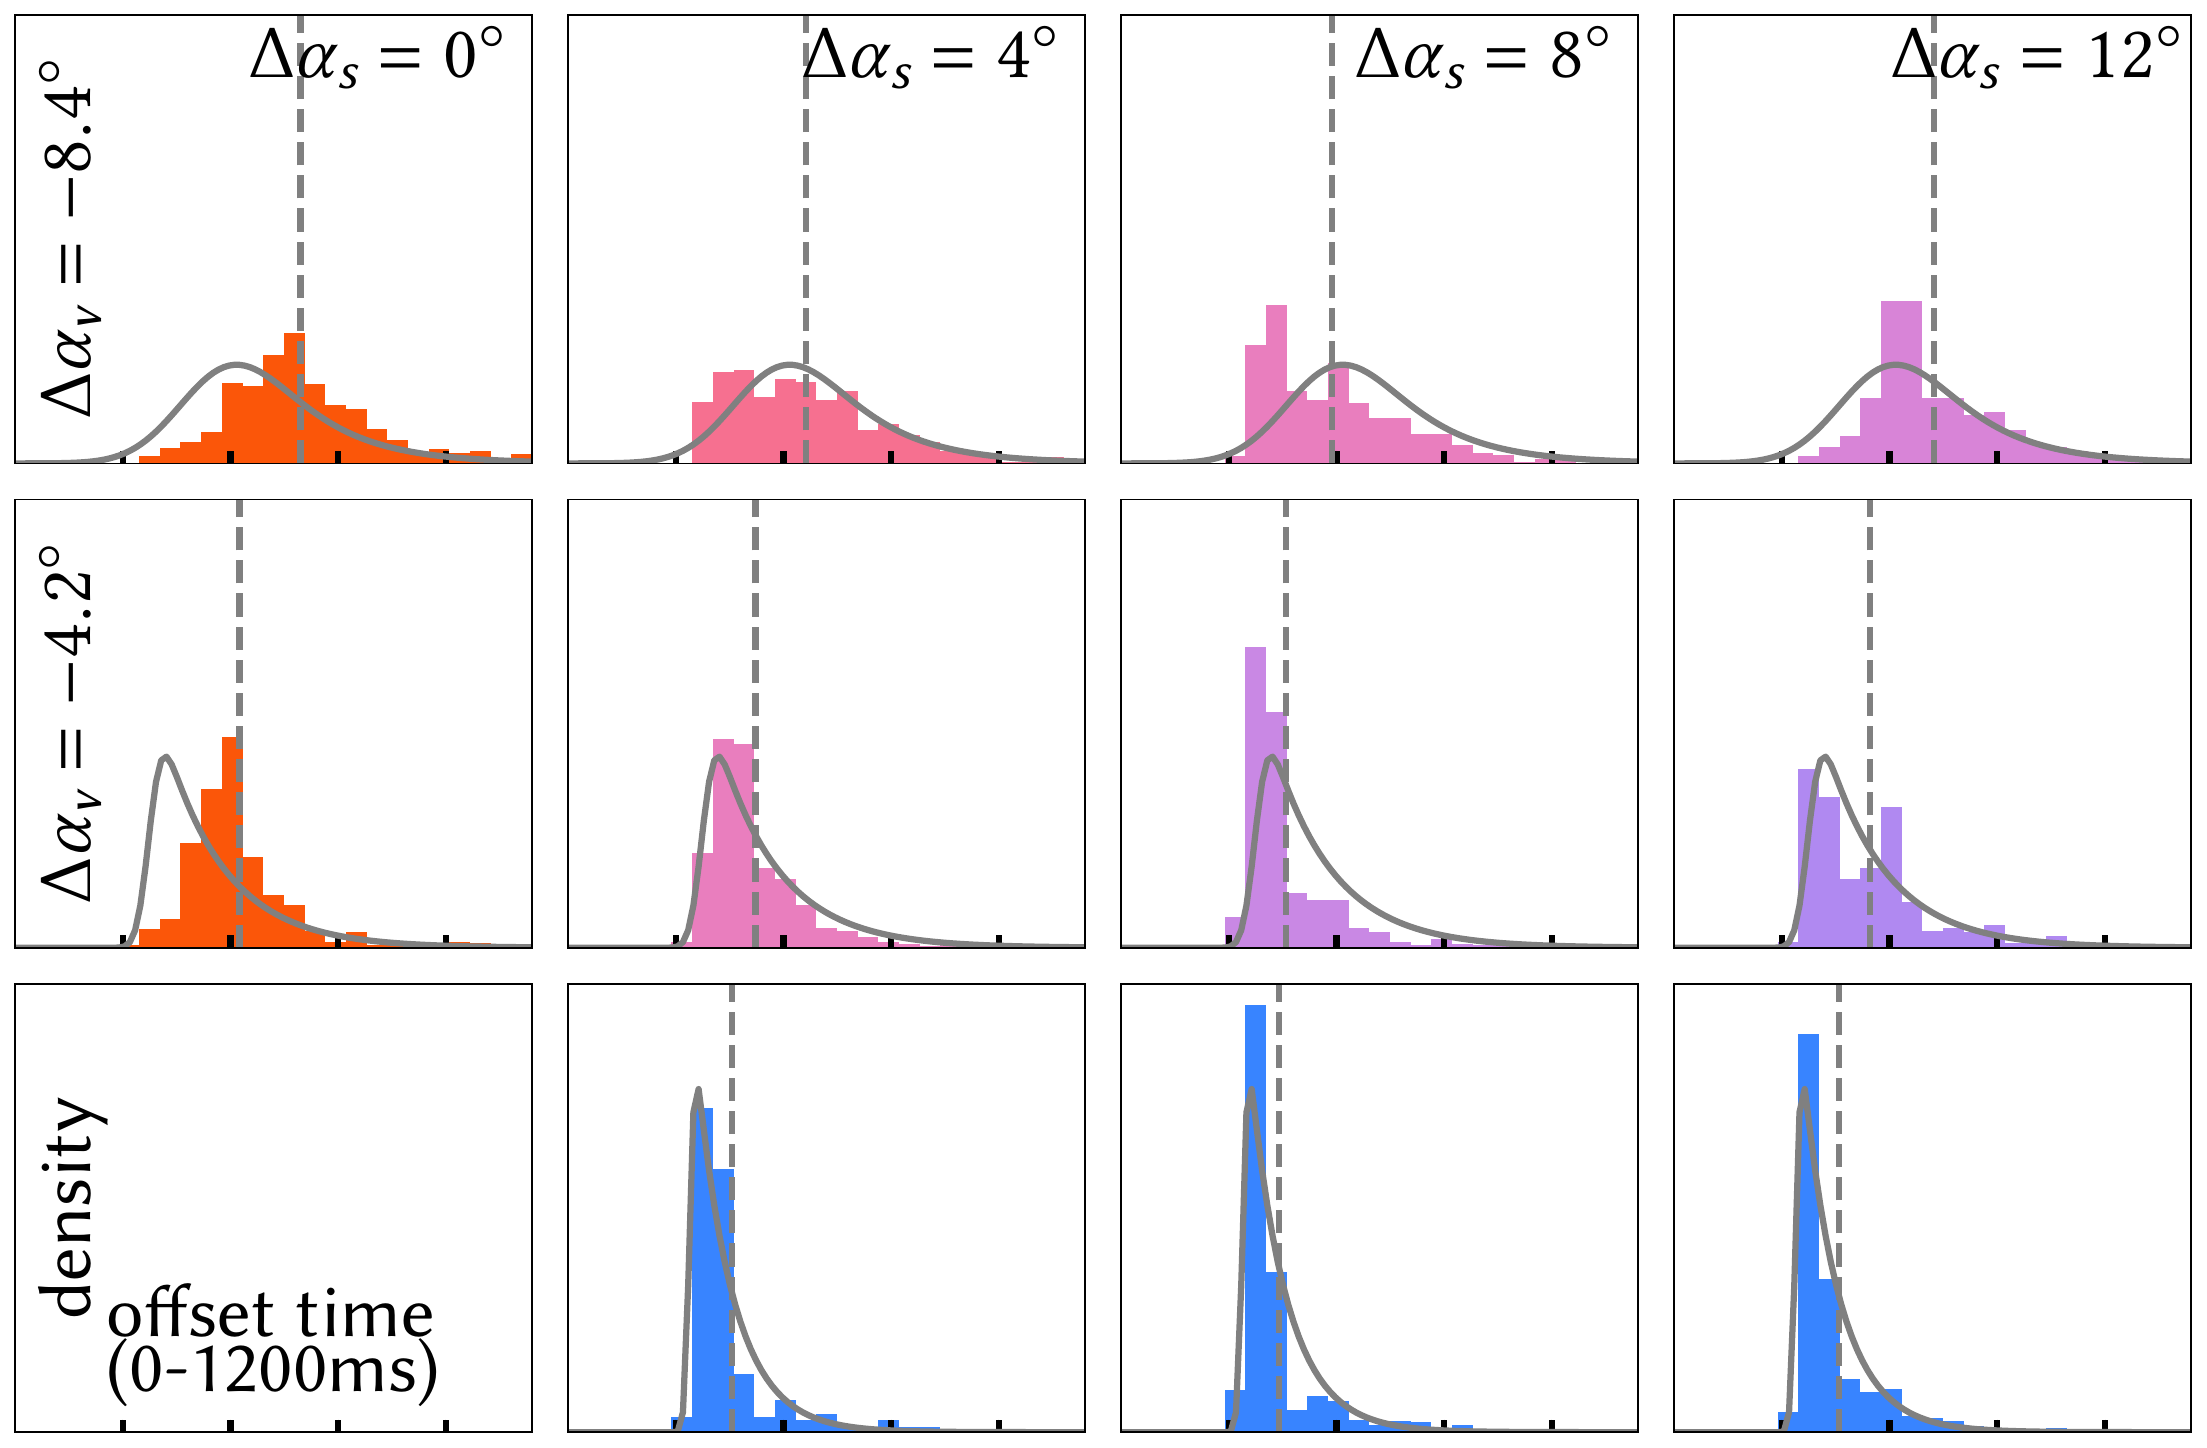}
        \label{fig:supp:ablation:vergence:div}
    }%subfloat
    \subfloat[$\conditionAccuracyVergence$, convergent]{
        \includegraphics[width=0.47\linewidth]{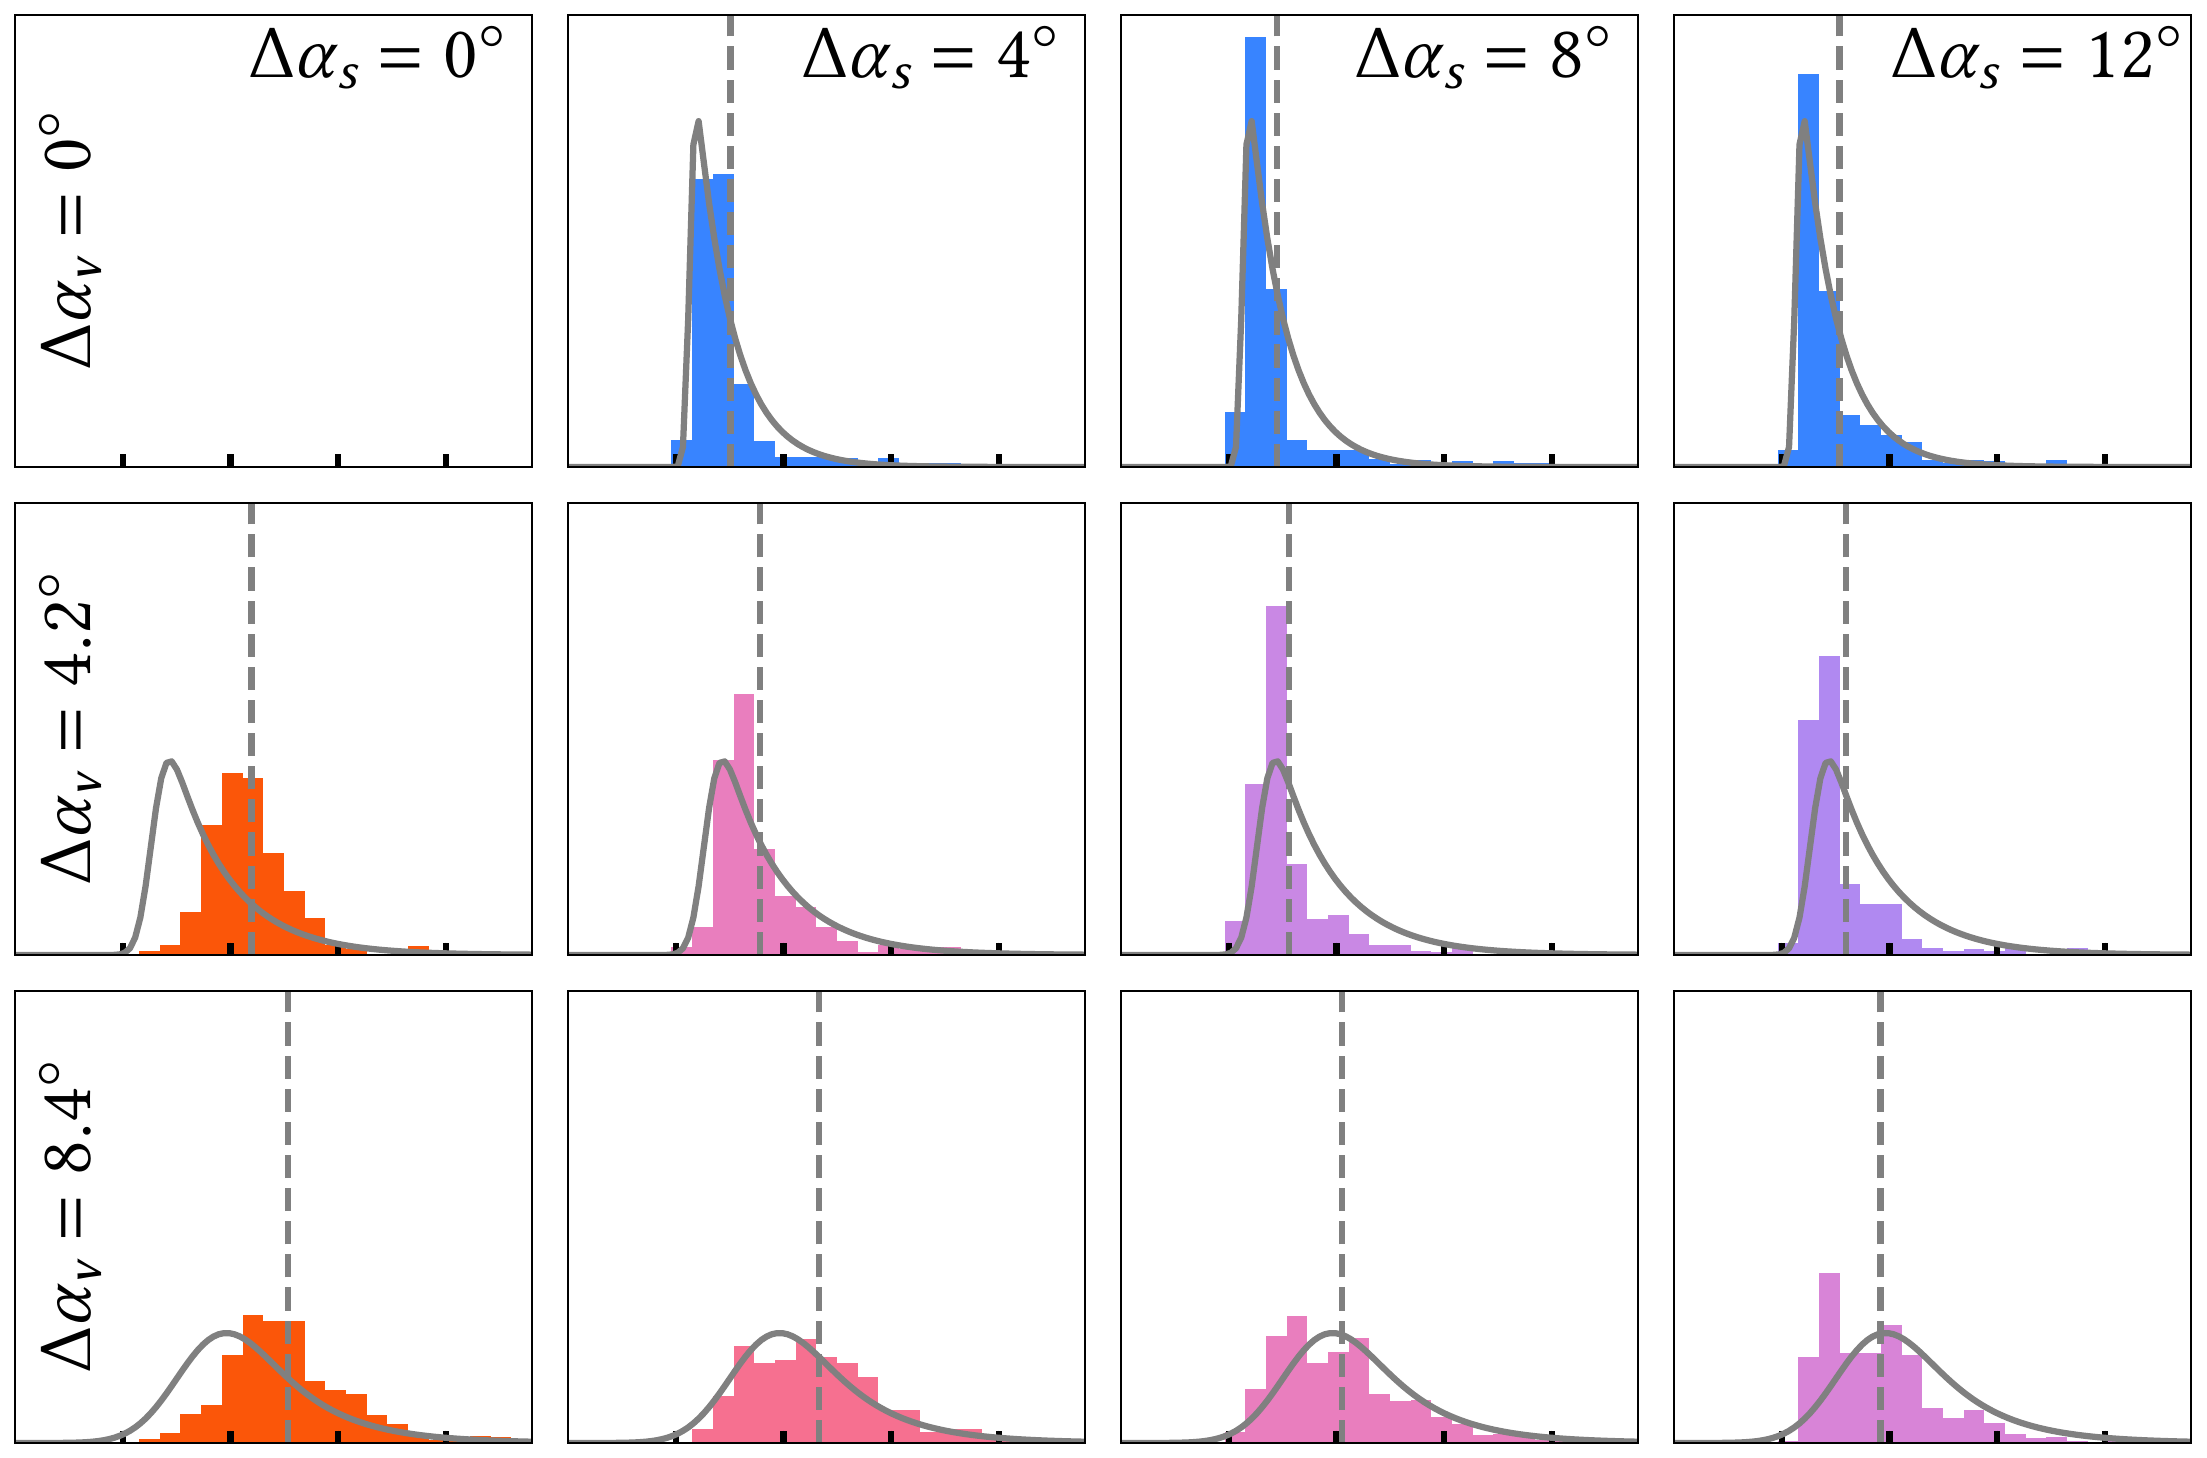}
        \label{fig:supp:ablation:vergence:con}
    }%subfloat
    
    \Caption{
        Histograms vs. predicted distributions of ablation models.
    }{
        Predicted distributions by the ablation models are compared to measured data from psychophysical study.
        Ablation model $\conditionAccuracySaccade$ was trained using only saccade amplitude information from the study data, while $\conditionAccuracyVergence$ only used vergence amplitude information.
        Since either model does not have full information that distinguishes individual conditions within a single column and row respectively, the models make the same predictions across multiple conditions within this histogram visualization.
        Thus, in \subref{fig:supp:ablation:saccade:div}/\subref{fig:supp:ablation:saccade:con} the model makes the same prediction within the same columns, while in \subref{fig:supp:ablation:vergence:div}/\subref{fig:supp:ablation:vergence:con} the model makes the same predictions within the same rows.
    }
\end{figure}
