# Supplementary material for: The Shortest Route Is Not Always the Fastest: Probability-Modeled Stereoscopic Eye Movement Completion Time in VR
Source: arXiv:2309.15183 source file (2023-10-03)
Supplement: Supplementary file 2 [file fig_supp_eval_tile.tex]

\begin{figure}[h]
    \centering
    \begin{tabular}{ m{0.06\linewidth} m{0.04\linewidth} m{0.04\linewidth} c c c }
        user & D & p & archery & basketball & natural\\        
        \hline
        \\
        $U_1$ & 0.2 & 1.0 & 
        \begin{minipage}{.095 \textwidth}
            \includegraphics[width=\linewidth]{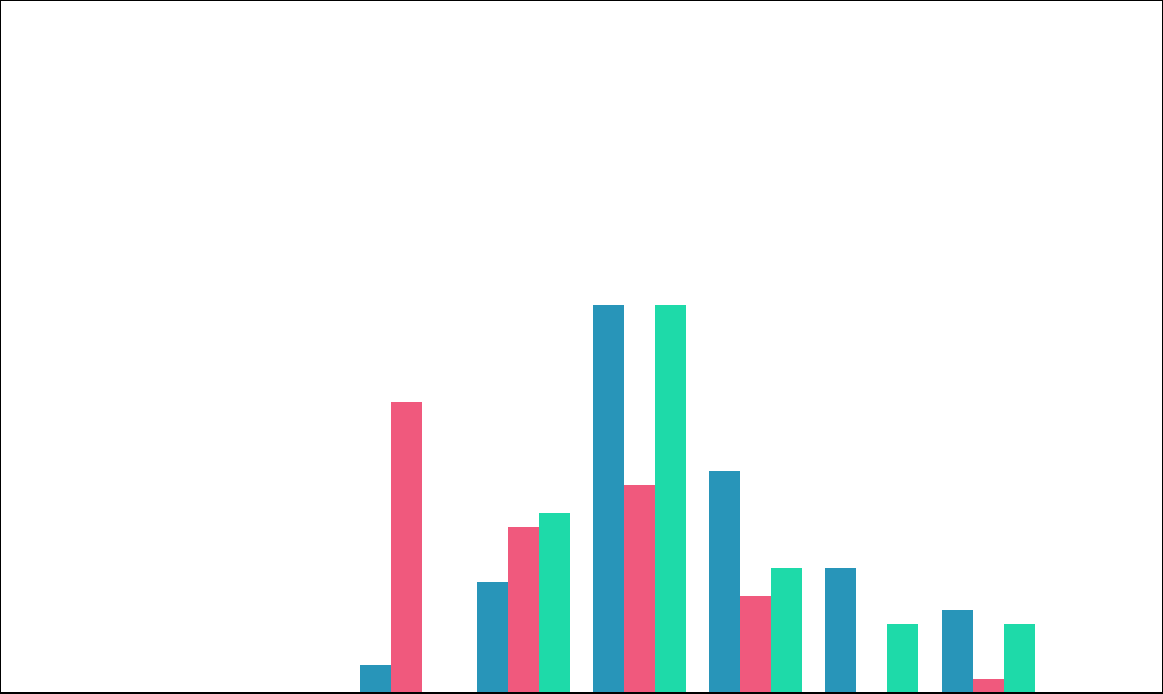}
        \end{minipage}
        &
        \begin{minipage}{.095 \textwidth}
            \includegraphics[width=\linewidth]{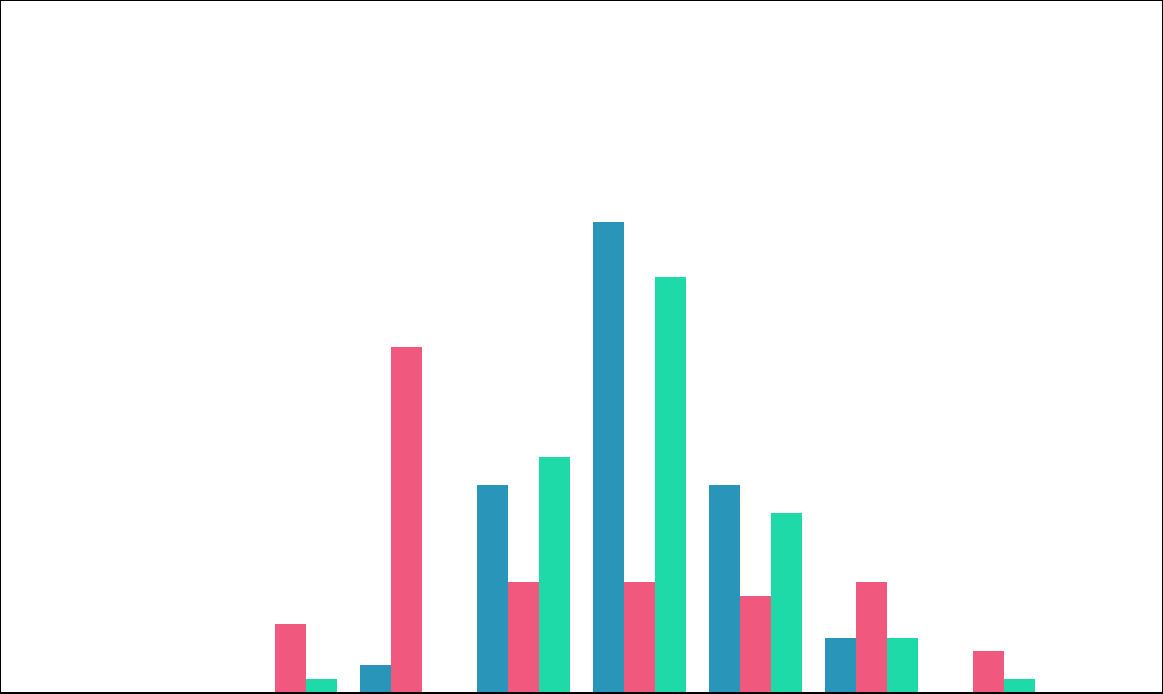}
        \end{minipage}
        &
        \begin{minipage}{.095 \textwidth}
            \includegraphics[width=\linewidth]{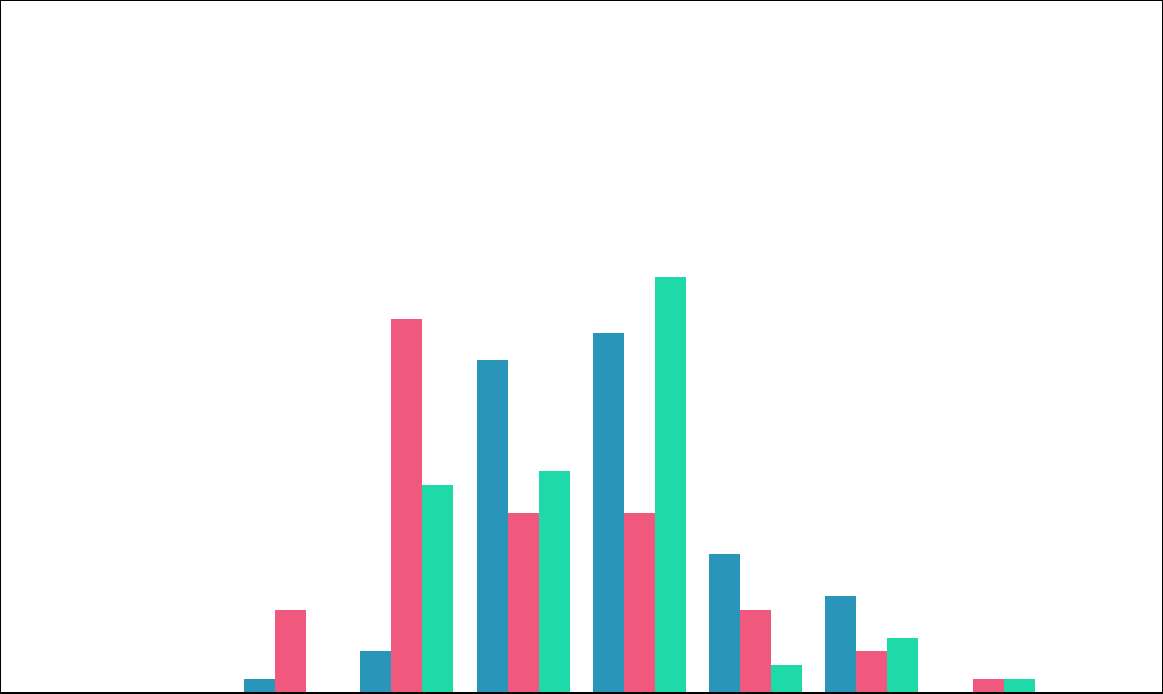}
        \end{minipage}
        \\ 
        
        $U_2$ & 0.3 & .79 &
        \begin{minipage}{.095 \textwidth}
            \includegraphics[width=\linewidth]{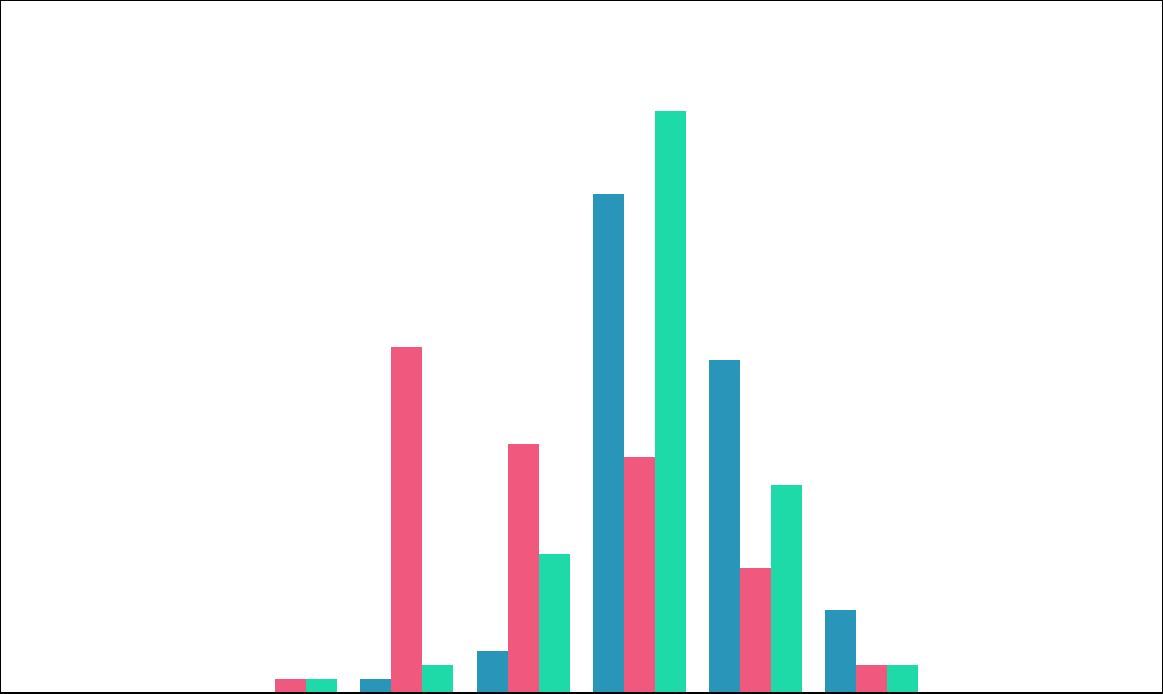}
        \end{minipage}
        &
        \begin{minipage}{.095 \textwidth}
            \includegraphics[width=\linewidth]{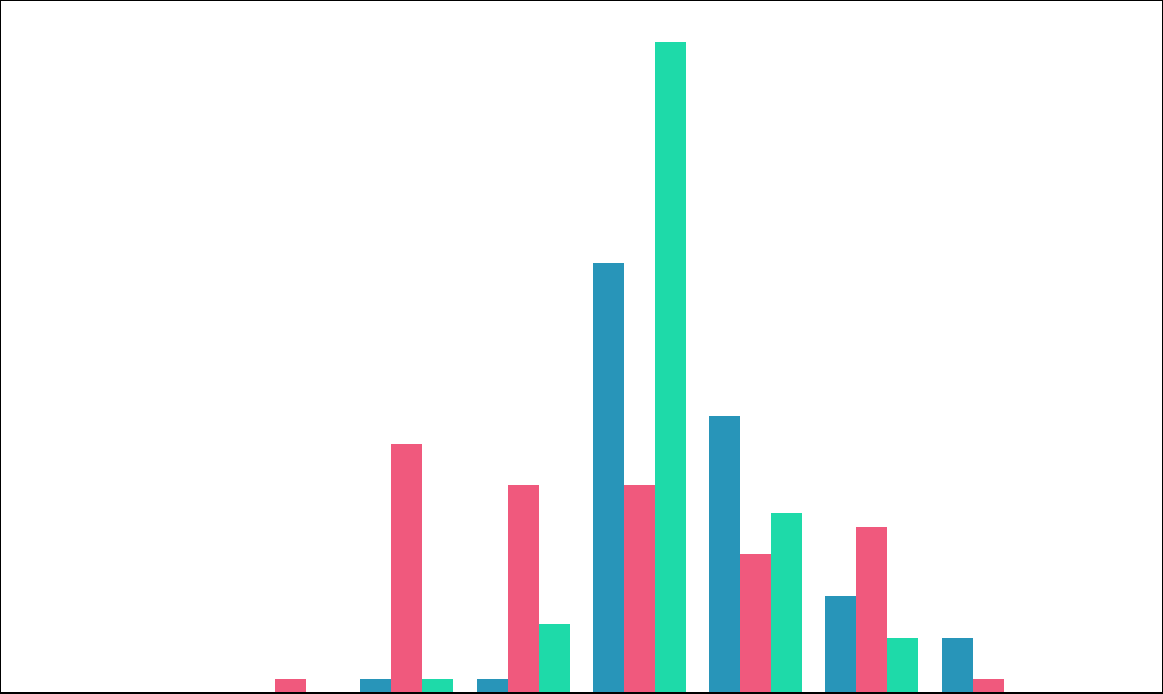}
        \end{minipage}
        &
        \begin{minipage}{.095 \textwidth}
            \includegraphics[width=\linewidth]{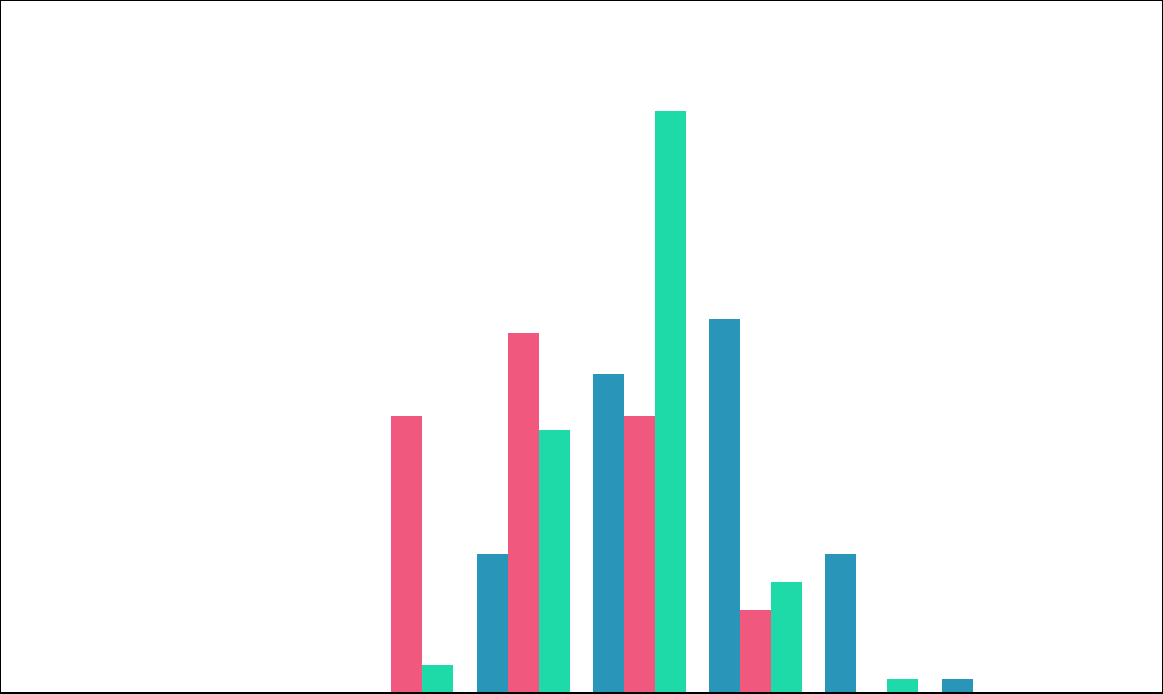}
        \end{minipage}
        \\    
        
        $U_3$ & 0.2 & 1.0&
        \begin{minipage}{.095 \textwidth}
            \includegraphics[width=\linewidth]{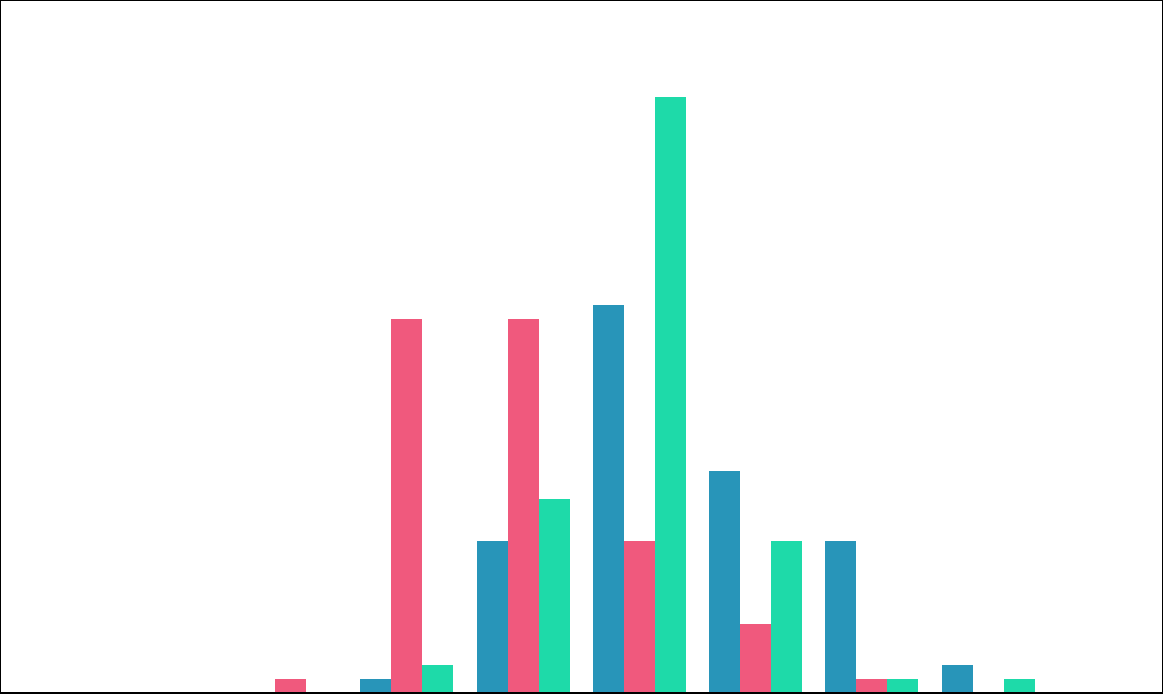}
        \end{minipage}
        &
        \begin{minipage}{.095 \textwidth}
            \includegraphics[width=\linewidth]{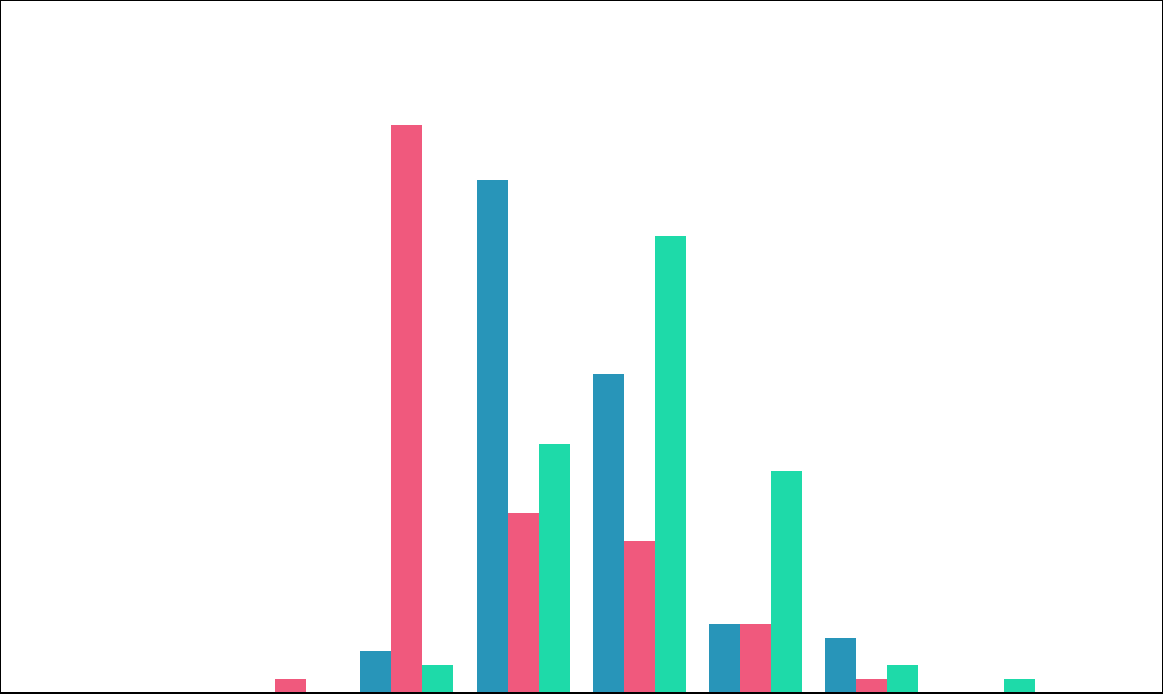}
        \end{minipage}
        &
        \begin{minipage}{.095 \textwidth}
            \includegraphics[width=\linewidth]{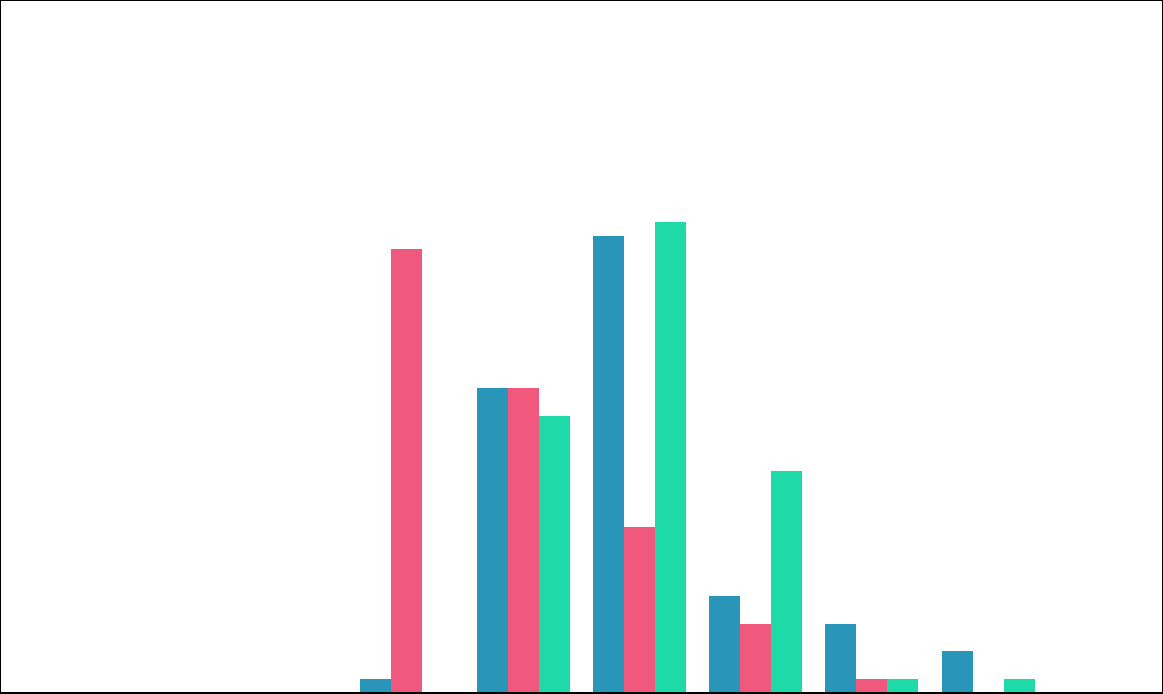}
        \end{minipage}
        \\  
        
        $U_4$ & 0.1& 1.0&
        \begin{minipage}{.095 \textwidth}
            \includegraphics[width=\linewidth]{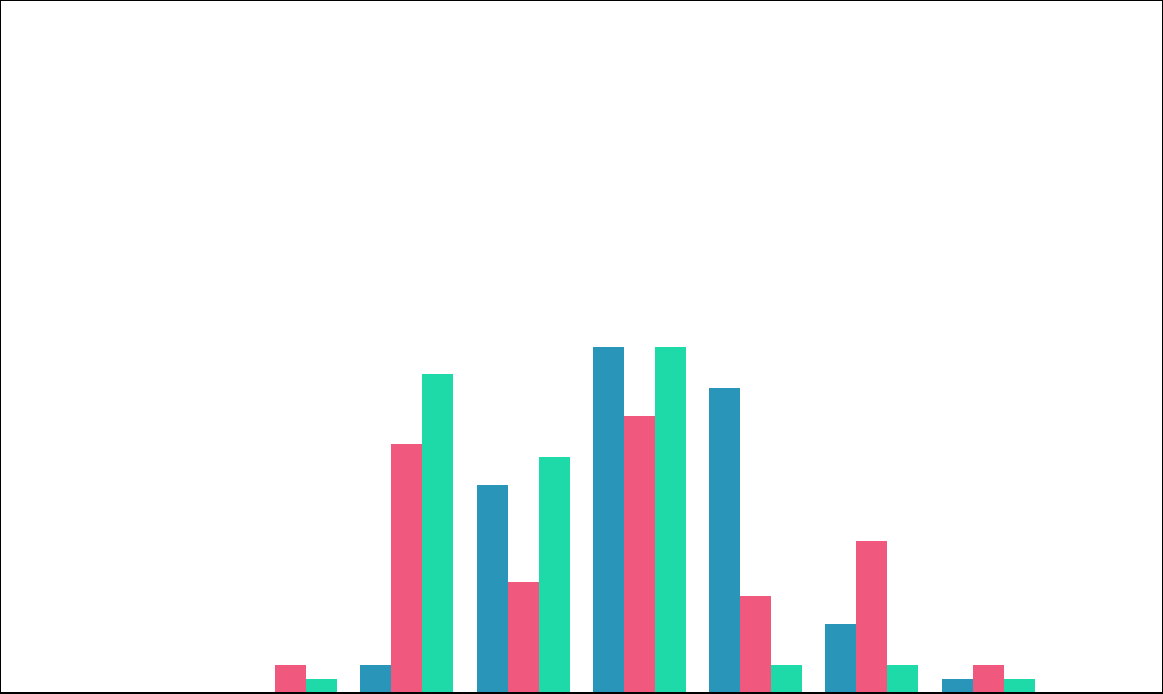}
        \end{minipage}
        &
        \begin{minipage}{.095 \textwidth}
            \includegraphics[width=\linewidth]{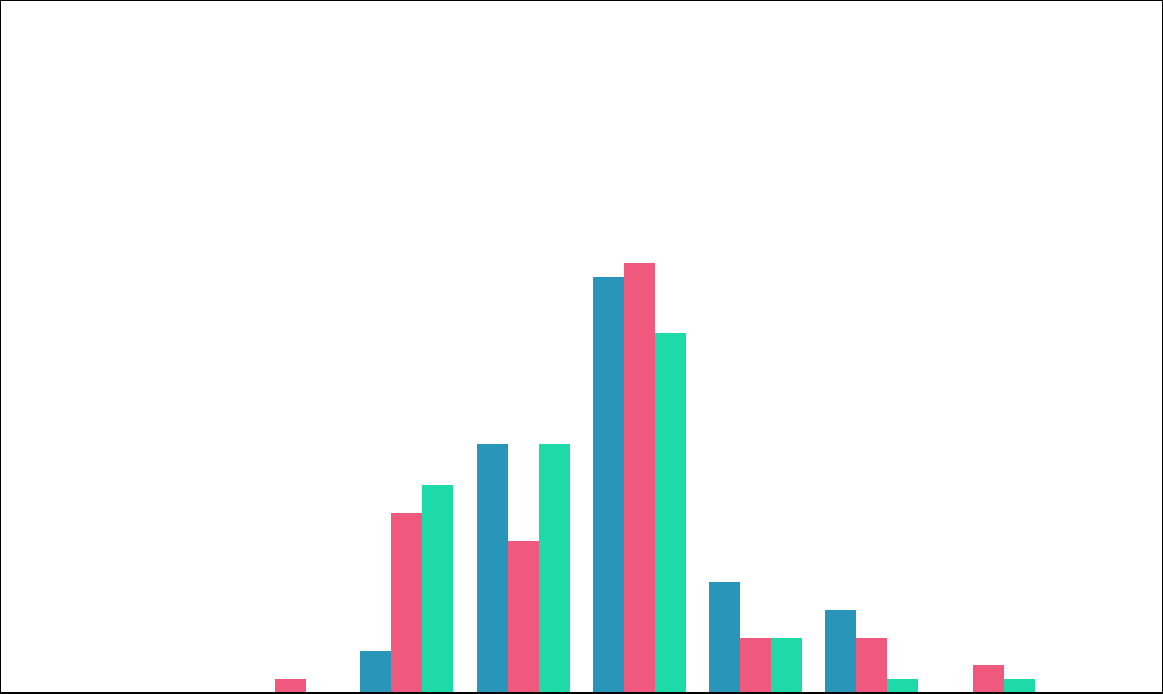}
        \end{minipage}
        &
        \begin{minipage}{.095 \textwidth}
            \includegraphics[width=\linewidth]{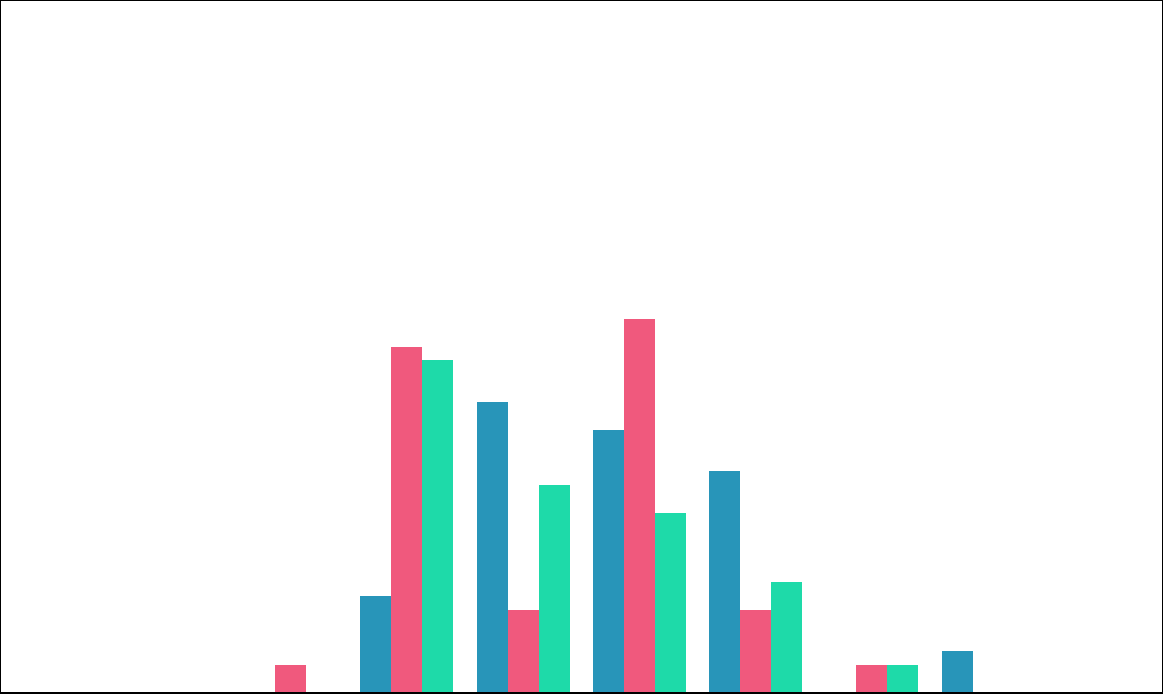}
        \end{minipage}
        \\  
        
        $U_5$ &0.2& 1.0&
        \begin{minipage}{.095 \textwidth}
            \includegraphics[width=\linewidth]{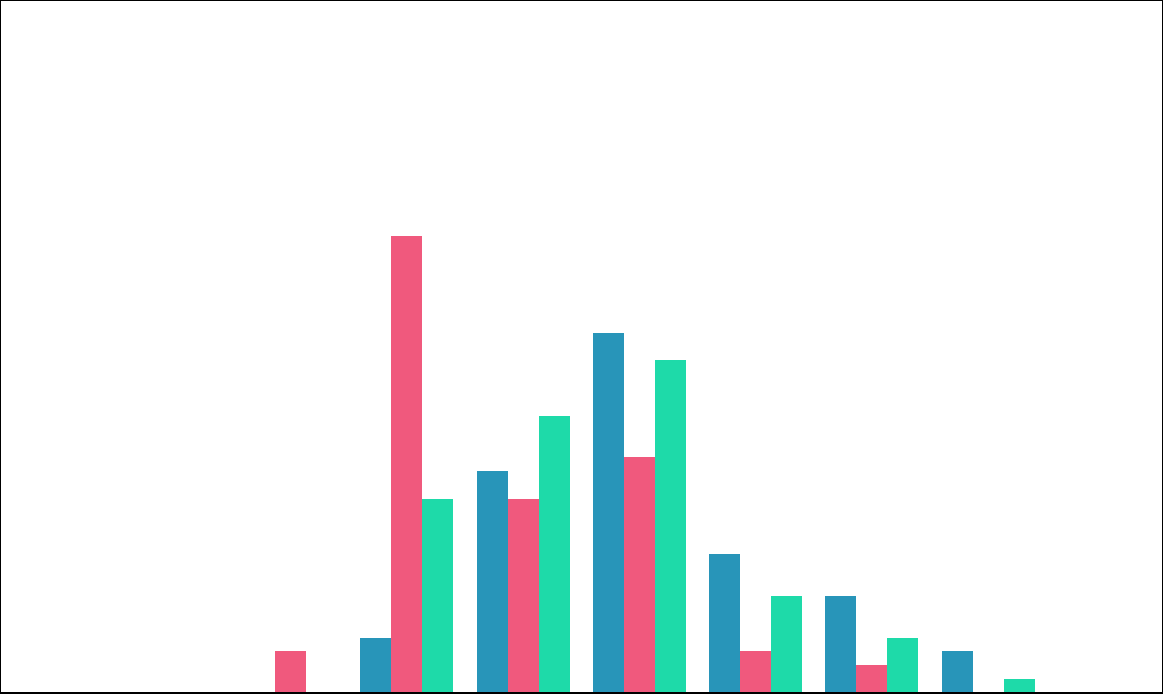}
        \end{minipage}
        &
        \begin{minipage}{.095 \textwidth}
            \includegraphics[width=\linewidth]{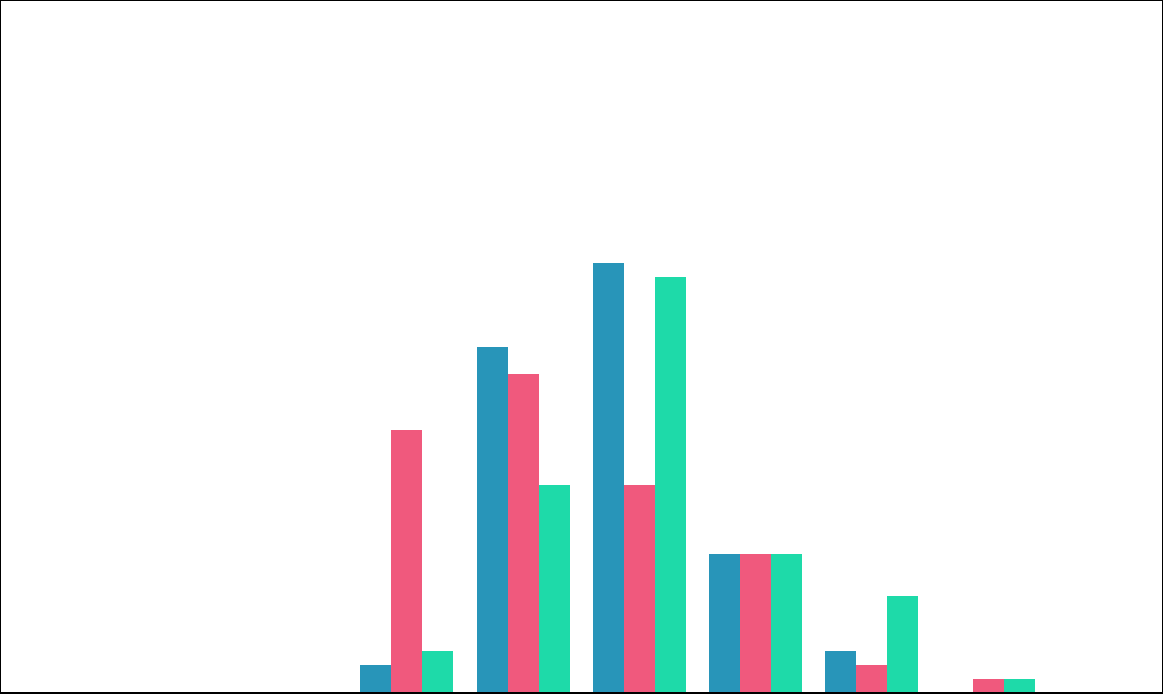}
        \end{minipage}
        &
        \begin{minipage}{.095 \textwidth}
            \includegraphics[width=\linewidth]{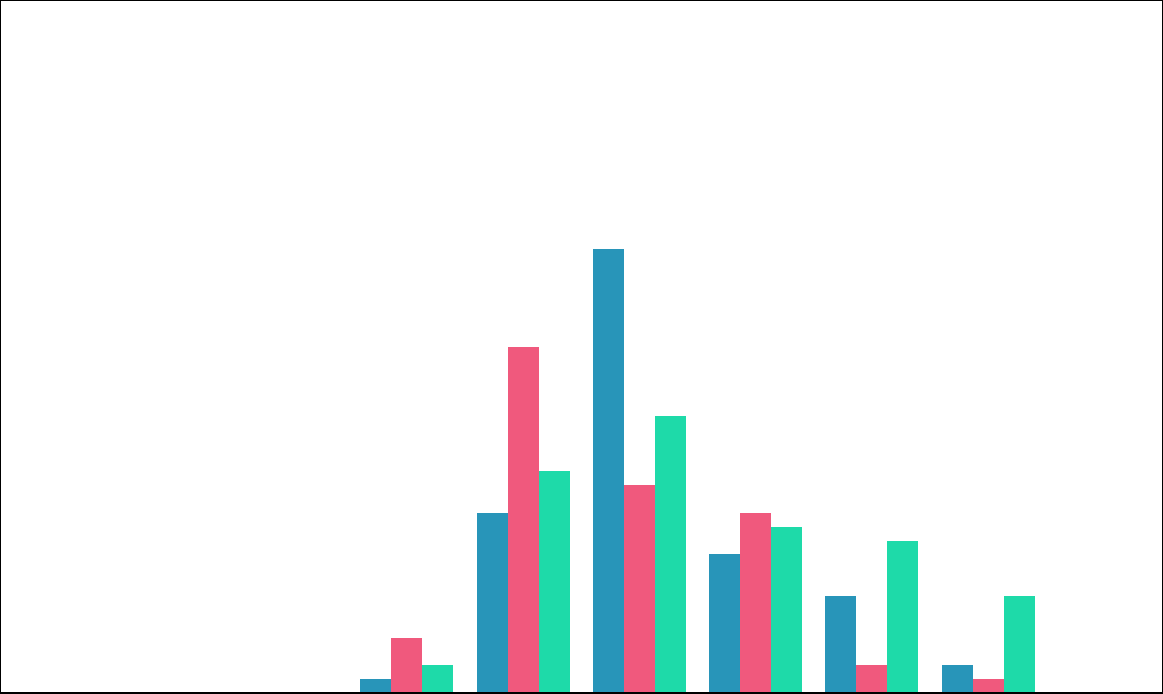}
        \end{minipage}
        \\  
        
        $U_6$ &0.1& 1.0&
        \begin{minipage}{.095 \textwidth}
            \includegraphics[width=\linewidth]{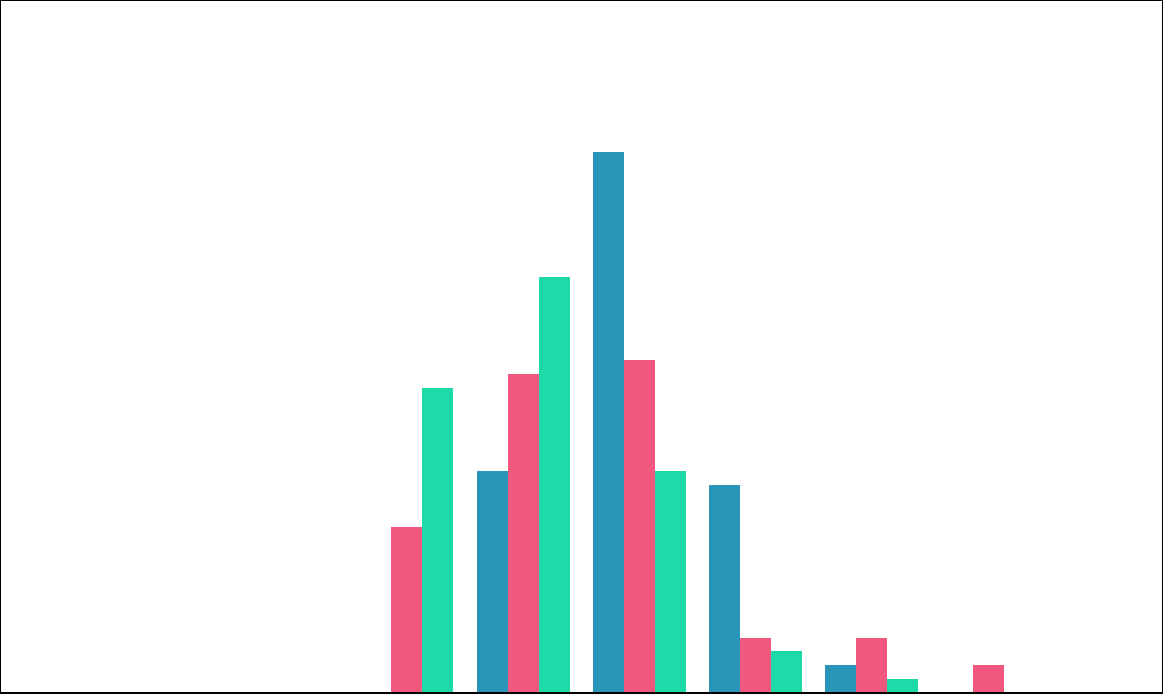}
        \end{minipage}
        &
        \begin{minipage}{.095 \textwidth}
            \includegraphics[width=\linewidth]{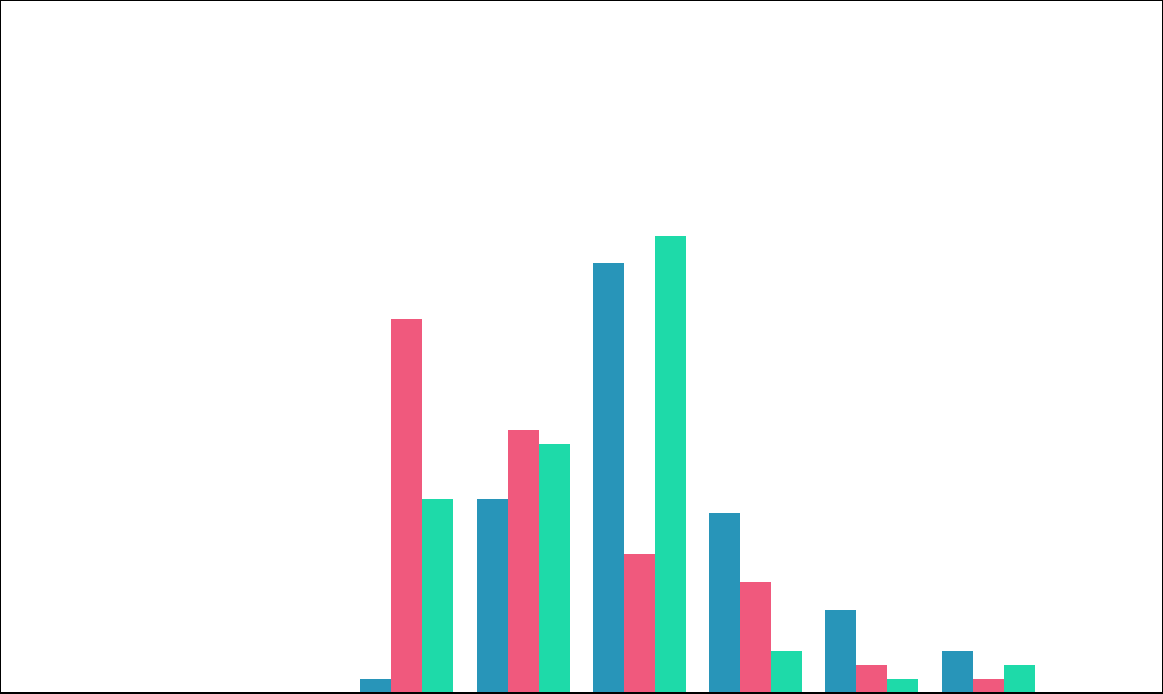}
        \end{minipage}
        &
        \begin{minipage}{.095 \textwidth}
            \includegraphics[width=\linewidth]{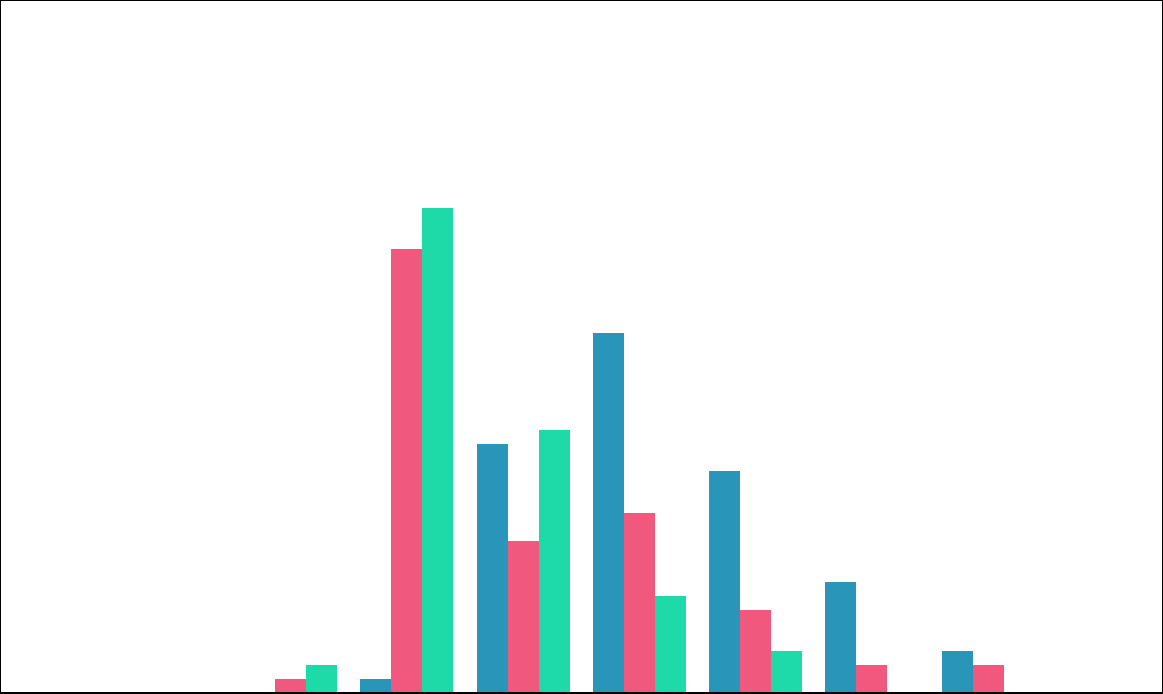}
        \end{minipage}
        \\         
        
        $U_7$ &0.1& 1.0&
        \begin{minipage}{.095 \textwidth}
            \includegraphics[width=\linewidth]{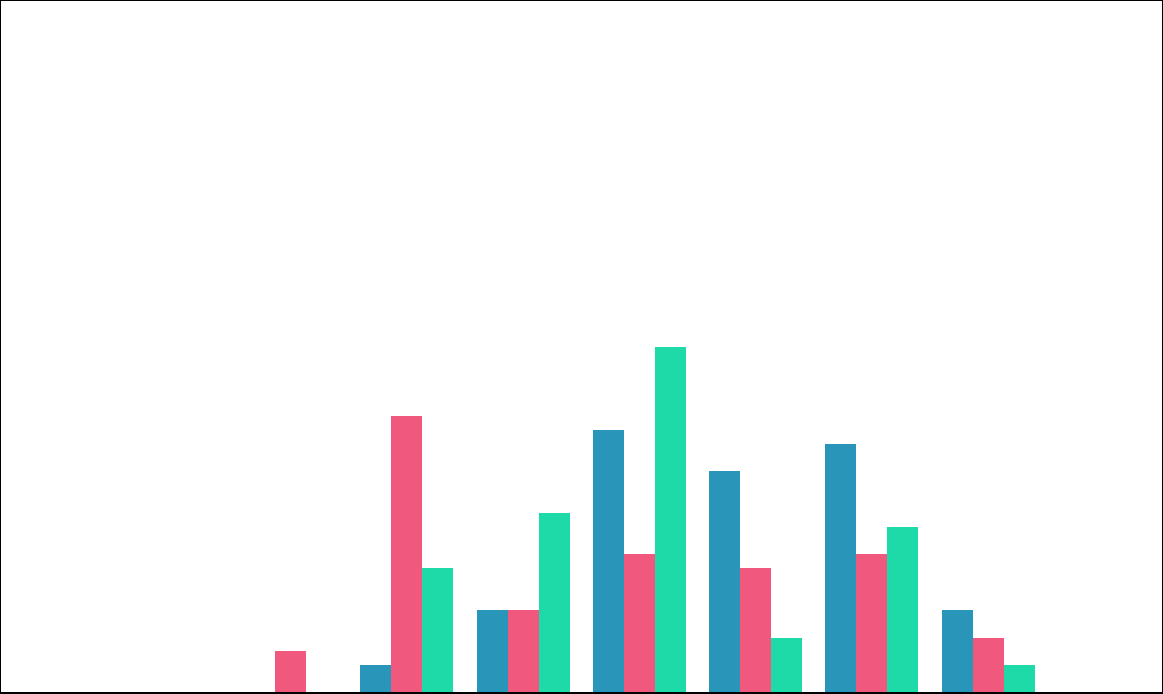}
        \end{minipage}
        &
        \begin{minipage}{.095 \textwidth}
            \includegraphics[width=\linewidth]{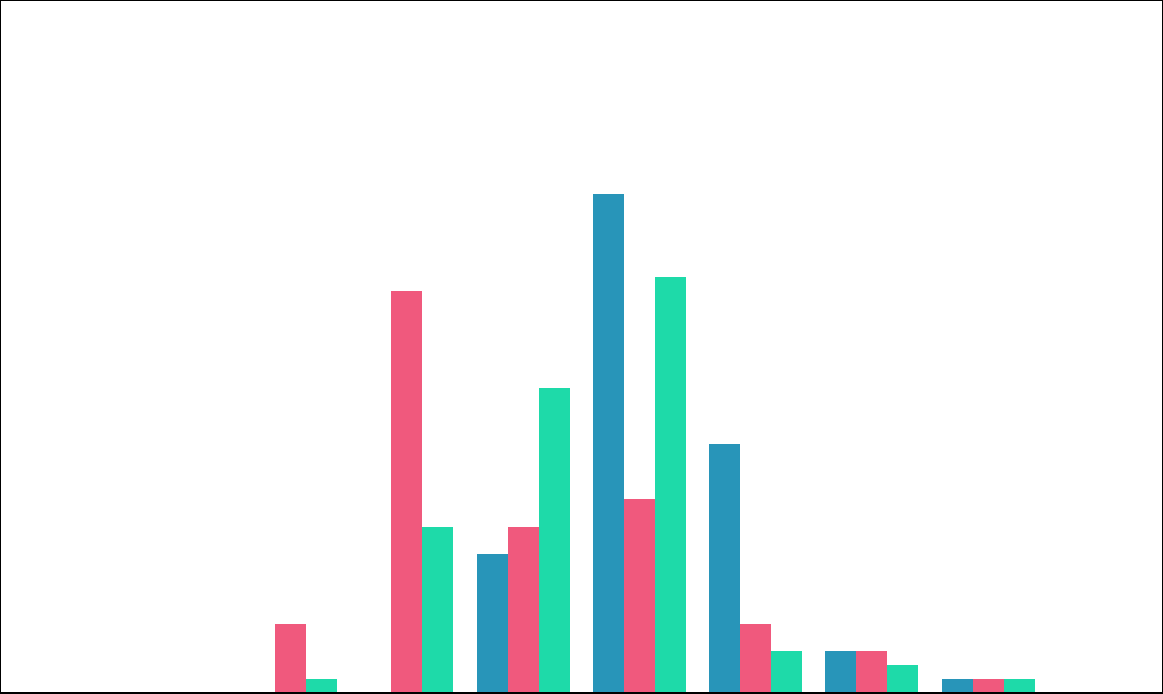}
        \end{minipage}
        &
        \begin{minipage}{.095 \textwidth}
            \includegraphics[width=\linewidth]{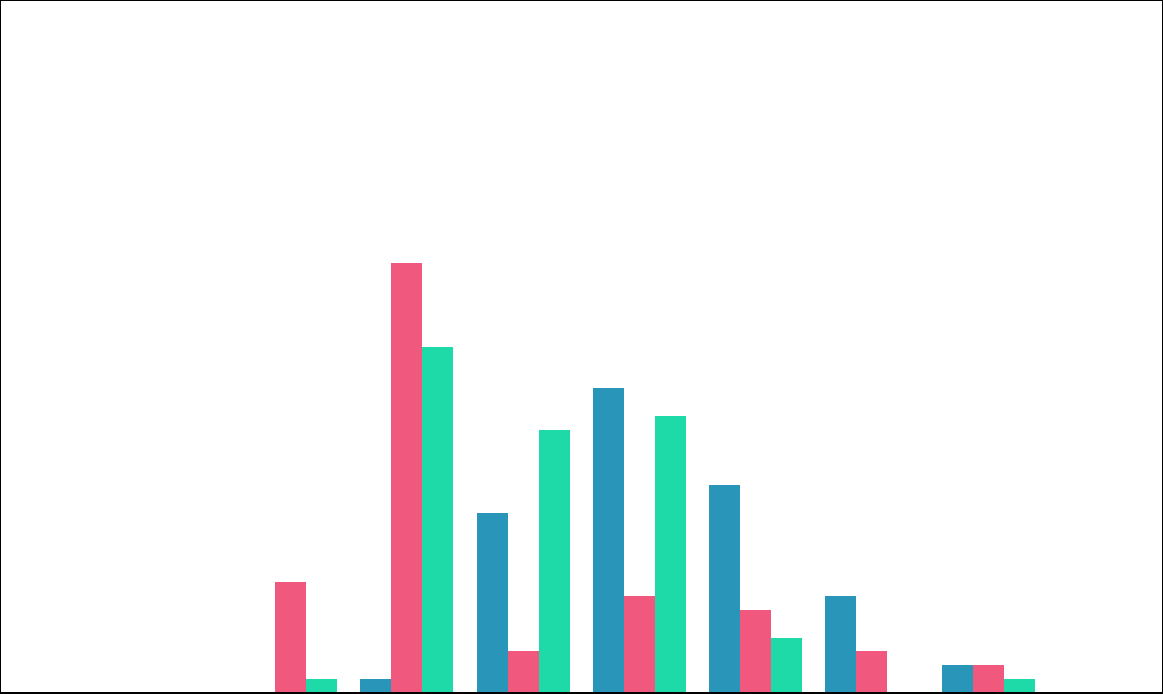}
        \end{minipage}
        \\  
        
        $U_8$ &0.2& 1.0&
        \begin{minipage}{.095 \textwidth}
            \includegraphics[width=\linewidth]{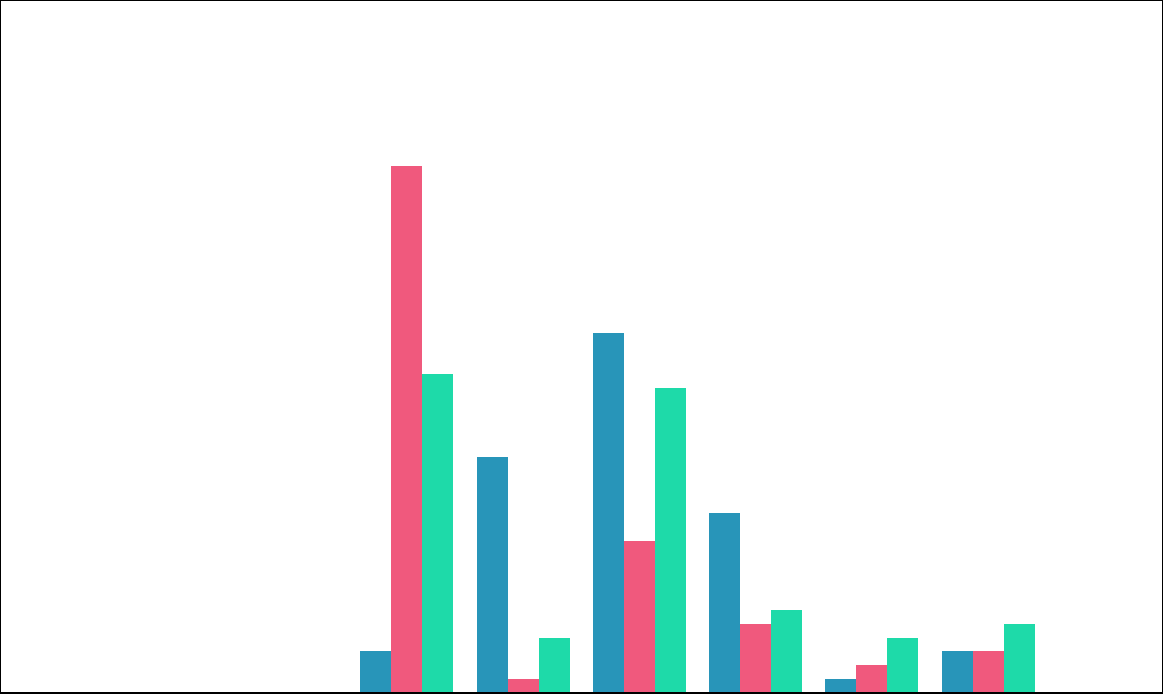}
        \end{minipage}
        &
        \begin{minipage}{.095 \textwidth}
            \includegraphics[width=\linewidth]{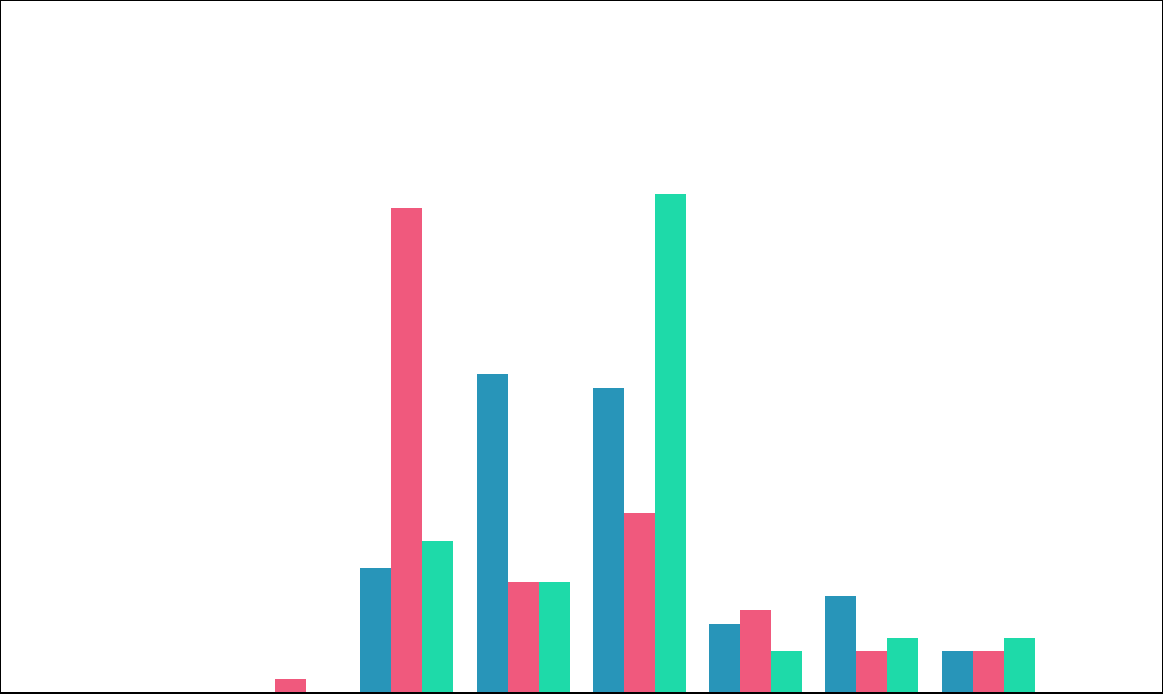}
        \end{minipage}
        &
        \begin{minipage}{.095 \textwidth}
            \includegraphics[width=\linewidth]{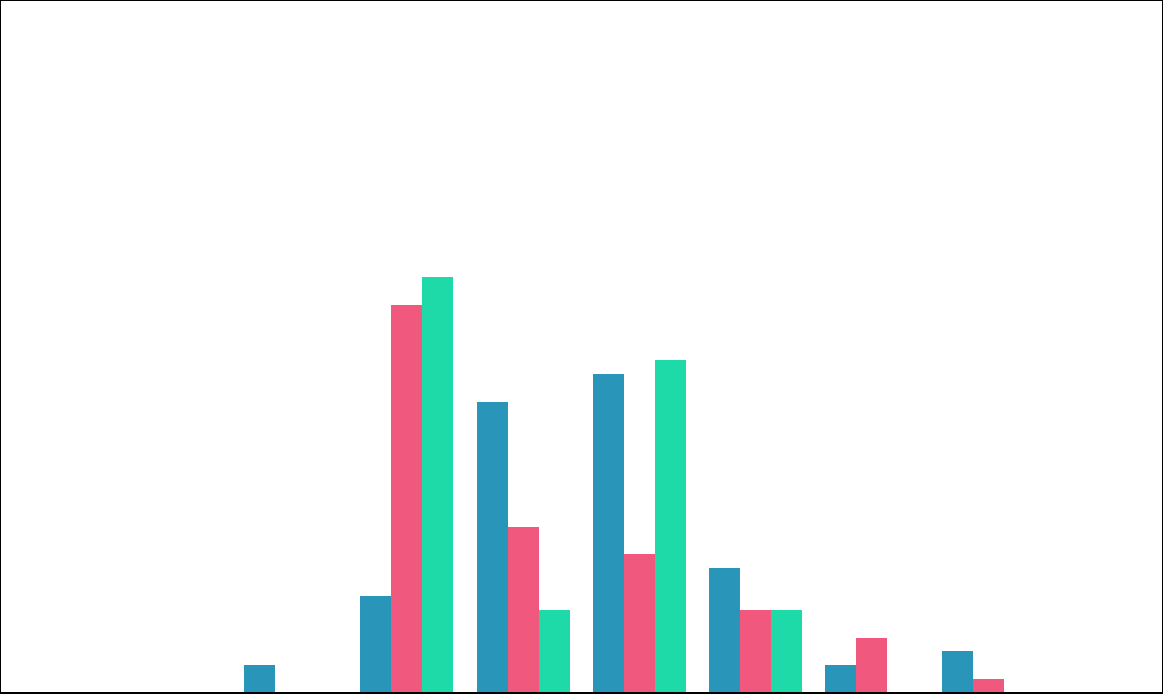}
        \end{minipage}
        \\  
        
        $U_9$ &0.1& 1.0&
        \begin{minipage}{.095 \textwidth}
            \includegraphics[width=\linewidth]{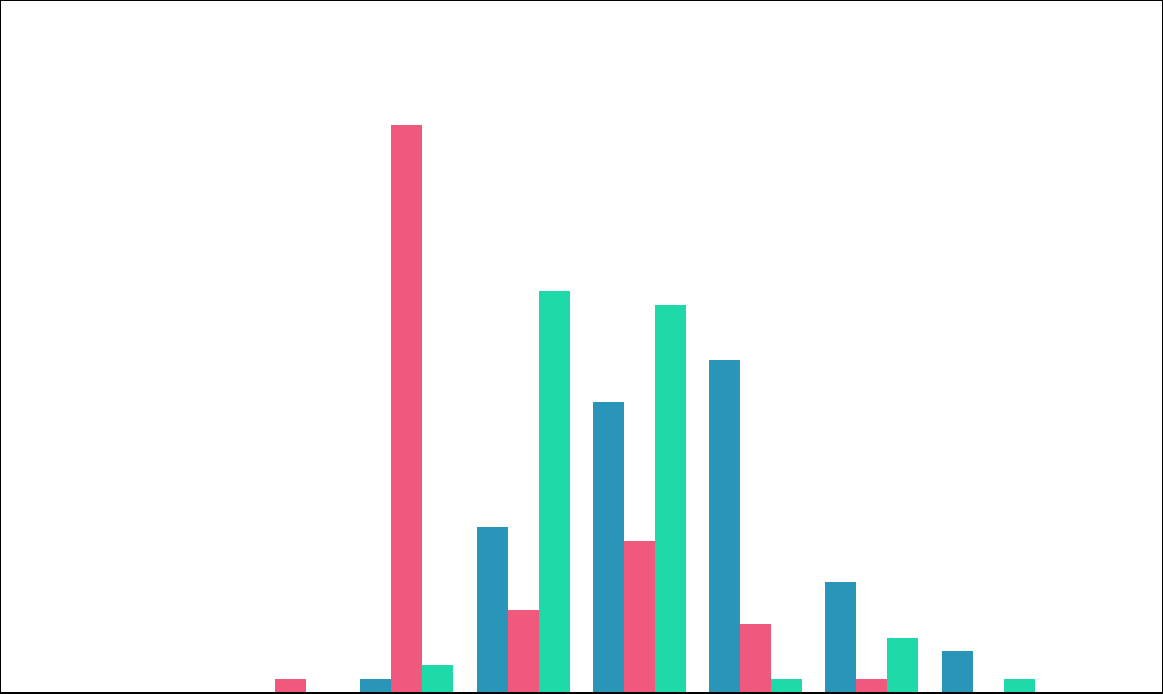}
        \end{minipage}
        &
        \begin{minipage}{.095 \textwidth}
            \includegraphics[width=\linewidth]{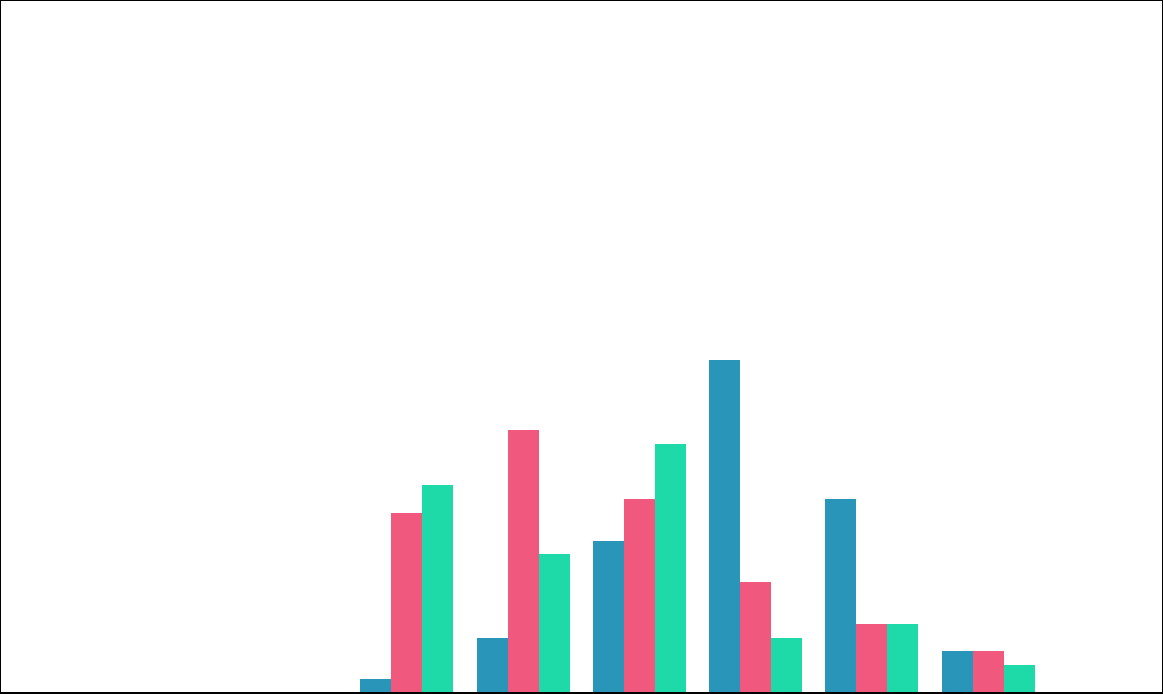}
        \end{minipage}
        &
        \begin{minipage}{.095 \textwidth}
            \includegraphics[width=\linewidth]{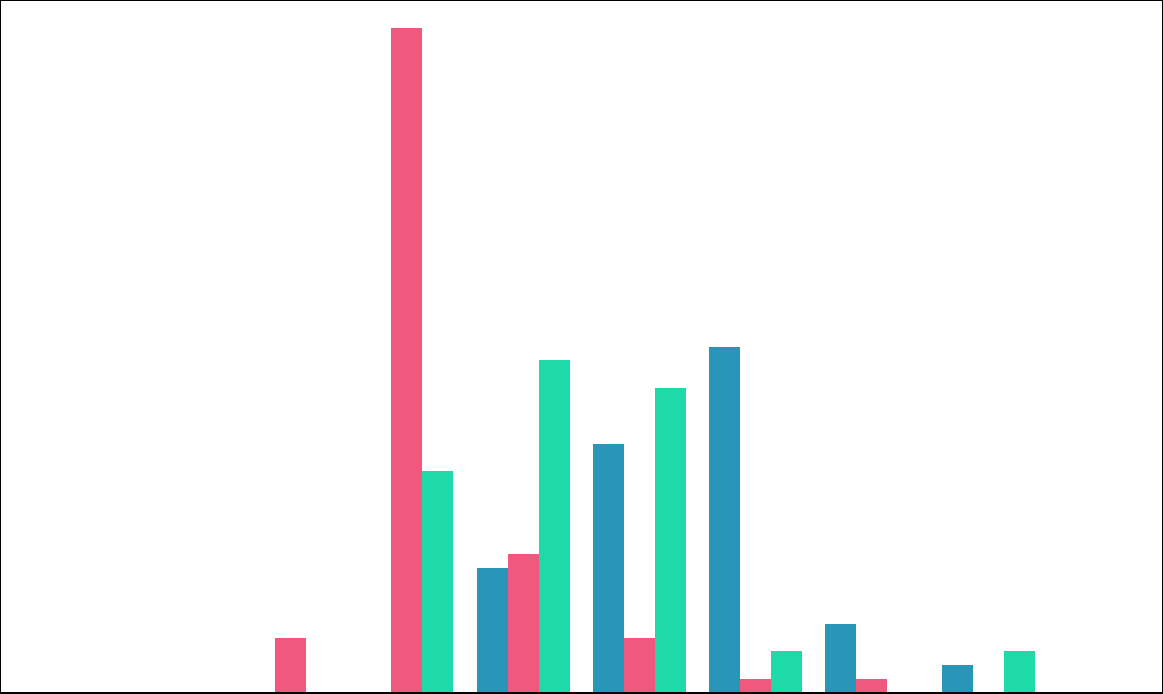}
        \end{minipage}
        \\  
        
        $U_{10}$ &0.2& 1.0&
        \begin{minipage}{.095 \textwidth}
            \includegraphics[width=\linewidth]{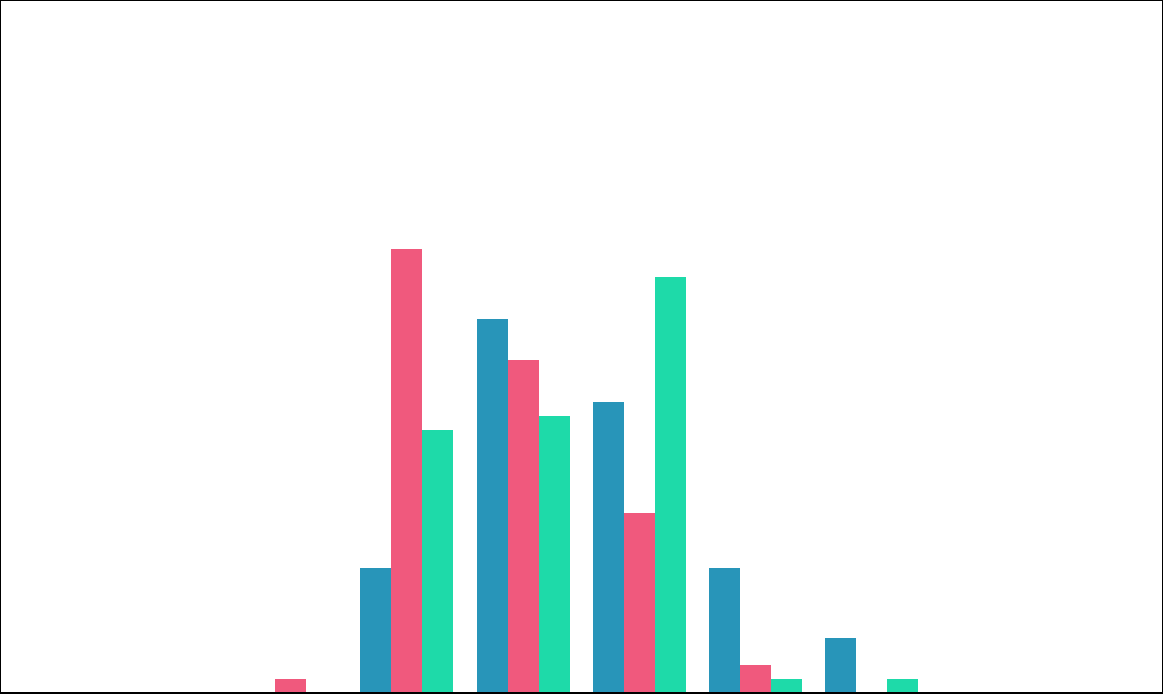}
        \end{minipage}
        &
        \begin{minipage}{.095 \textwidth}
            \includegraphics[width=\linewidth]{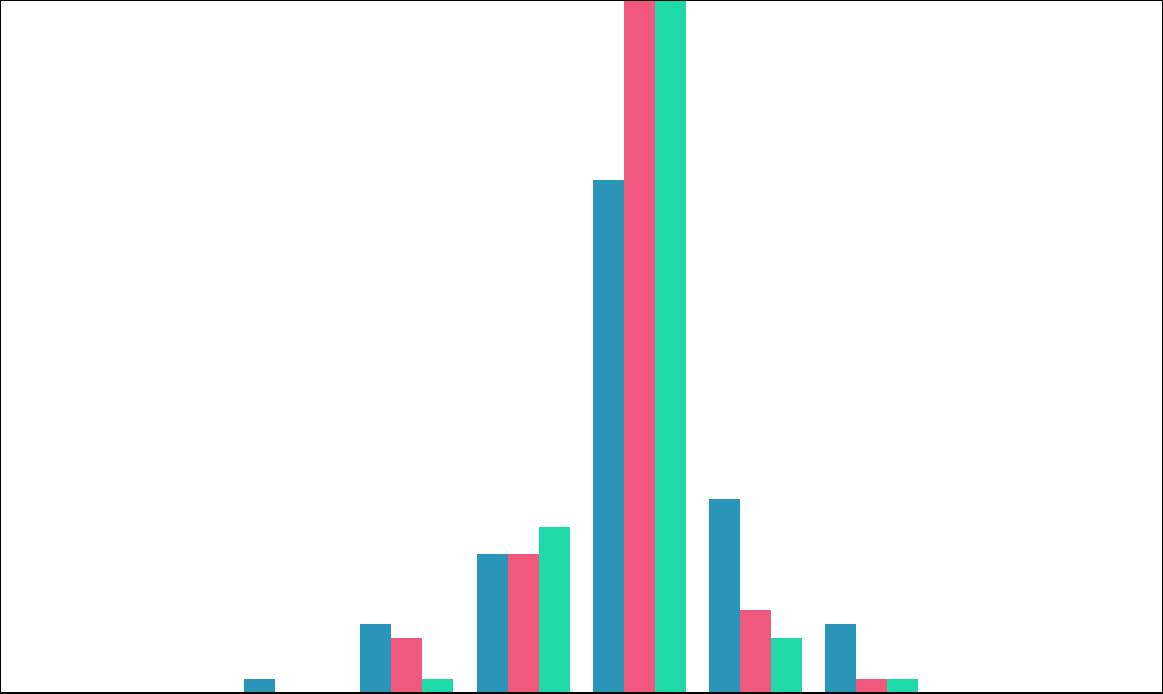}
        \end{minipage}
        &
        \begin{minipage}{.095 \textwidth}
            \includegraphics[width=\linewidth]{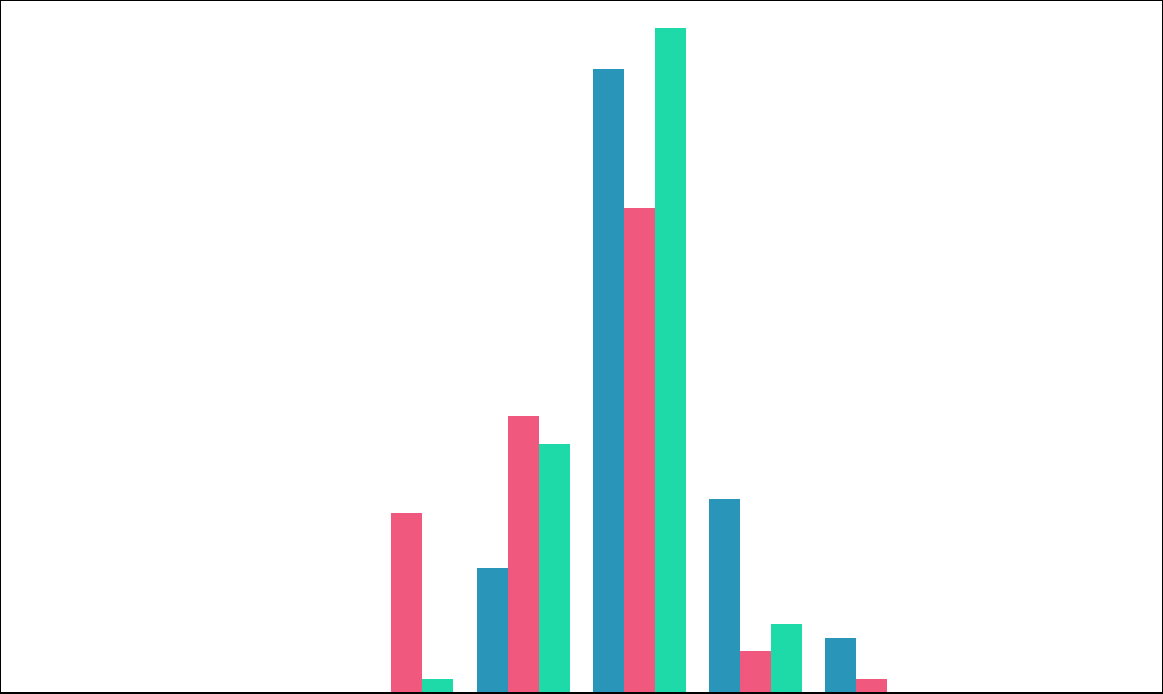}
        \end{minipage}
        \\       
        
        $U_{11}$ &0.2& 1.0&
        \begin{minipage}{.095 \textwidth}
            \includegraphics[width=\linewidth]{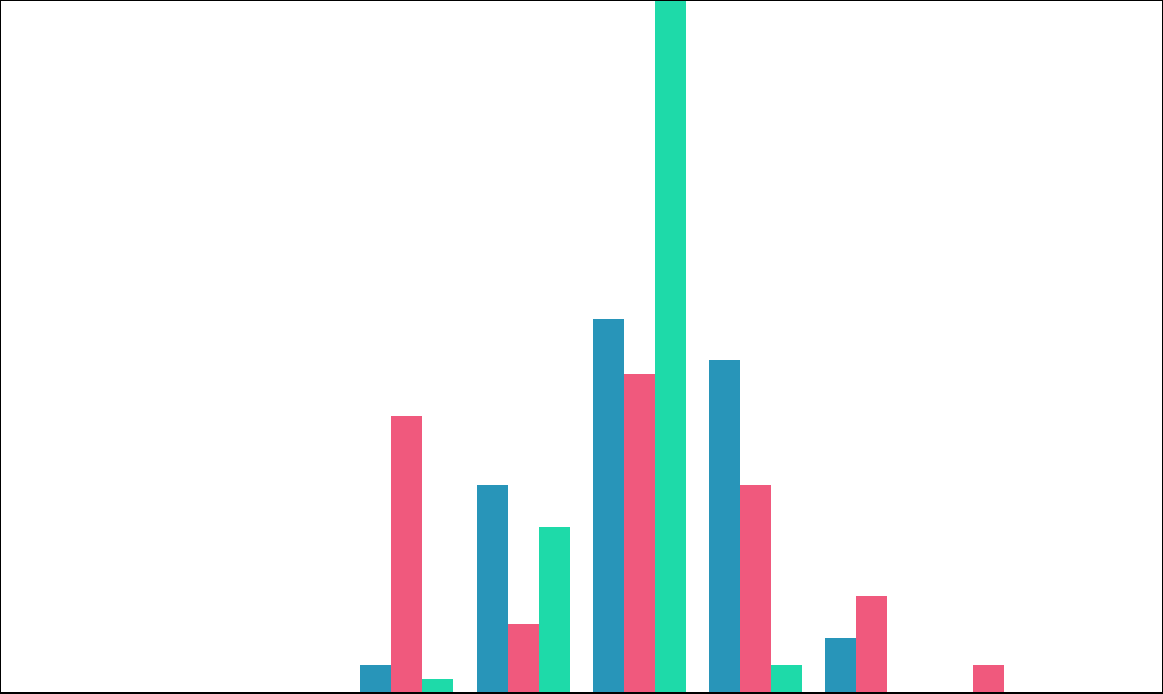}
        \end{minipage}
        &
        \begin{minipage}{.095 \textwidth}
            \includegraphics[width=\linewidth]{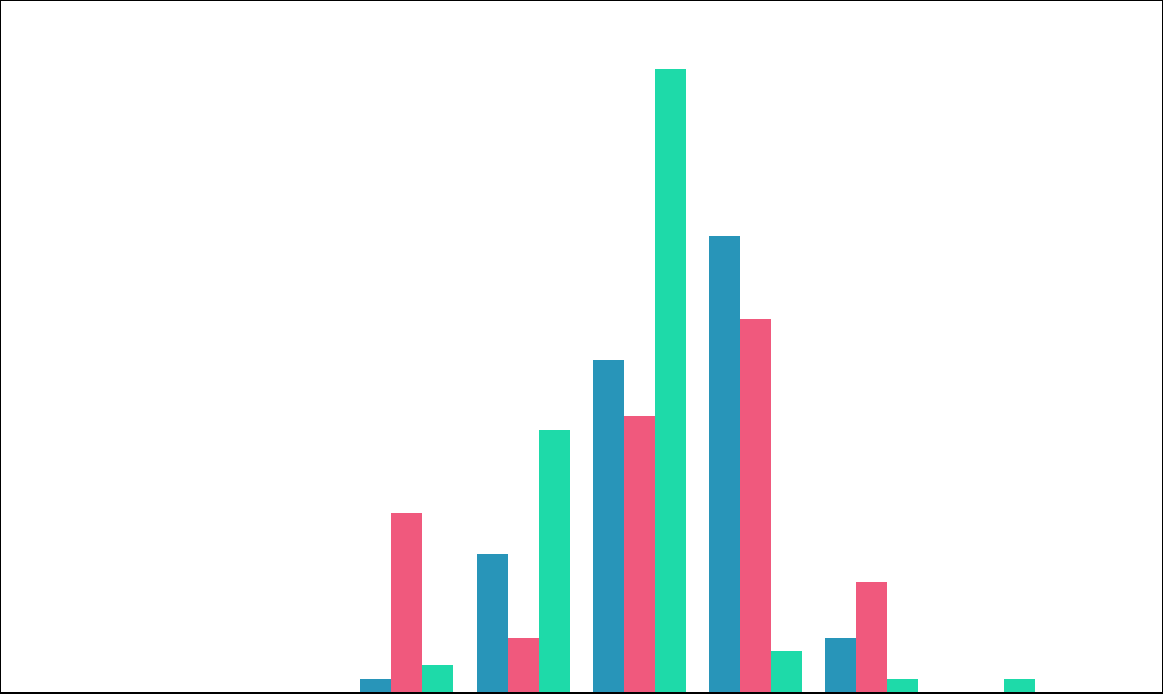}
        \end{minipage}
        &
        \begin{minipage}{.095 \textwidth}
            \includegraphics[width=\linewidth]{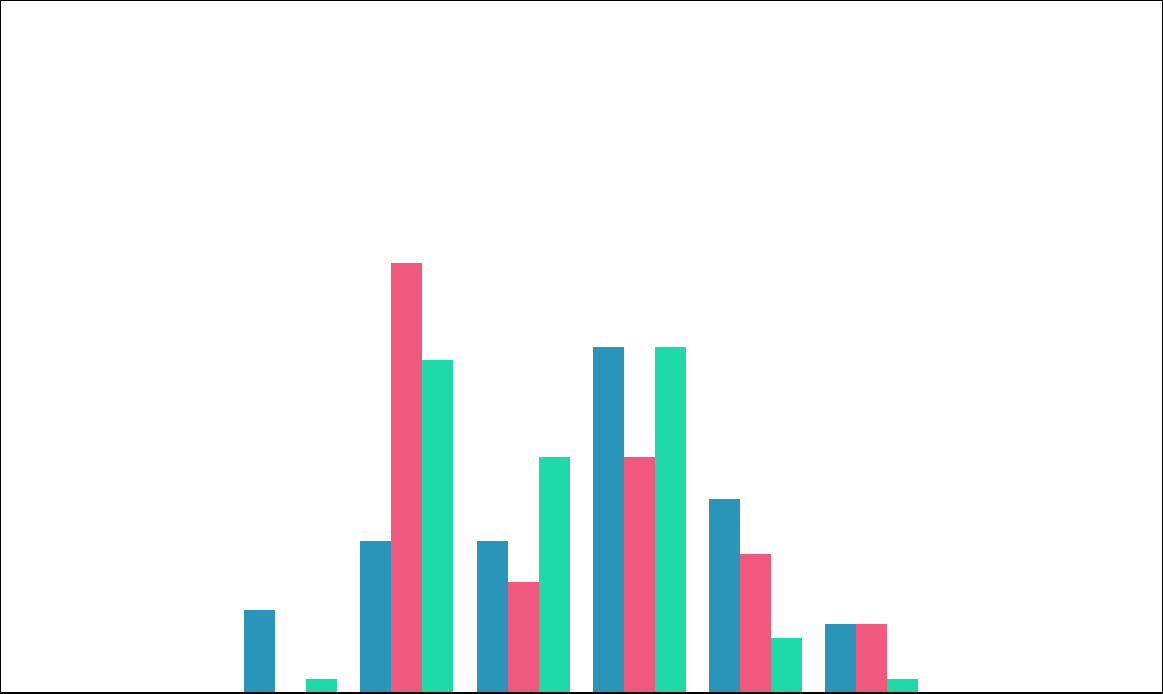}
        \end{minipage}
        \\          
        
        $U_{12}$ &0.2& 1.0&
        \begin{minipage}{.095 \textwidth}
            \includegraphics[width=\linewidth]{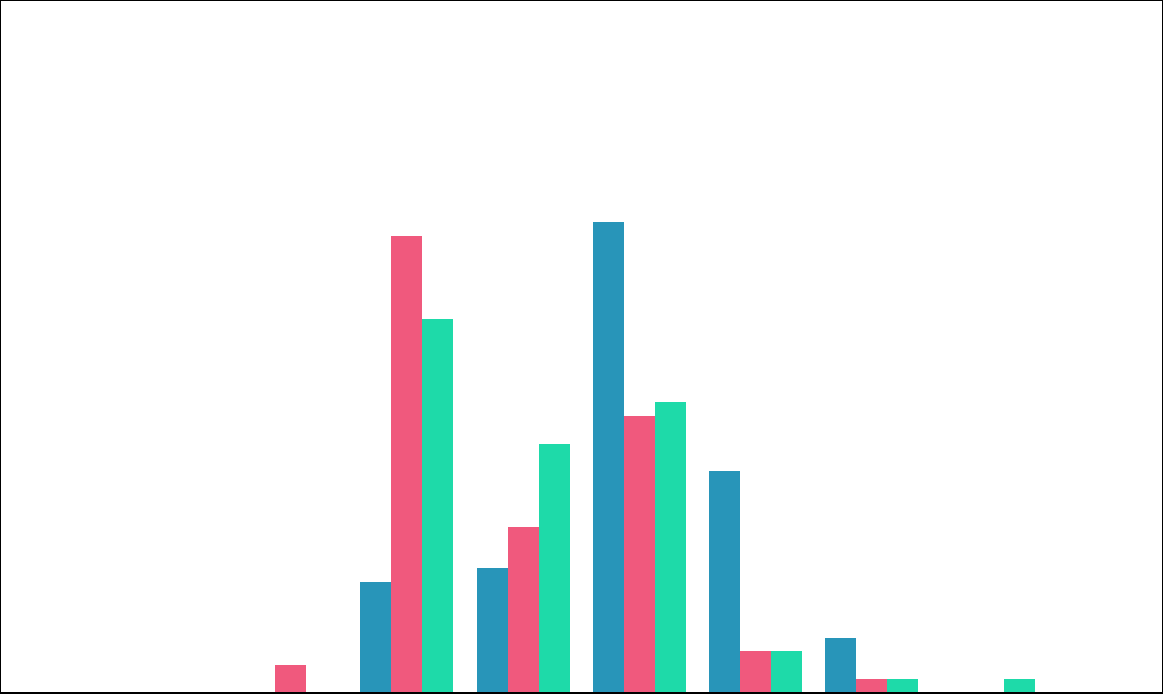}
        \end{minipage}
        &
        \begin{minipage}{.095 \textwidth}
            \includegraphics[width=\linewidth]{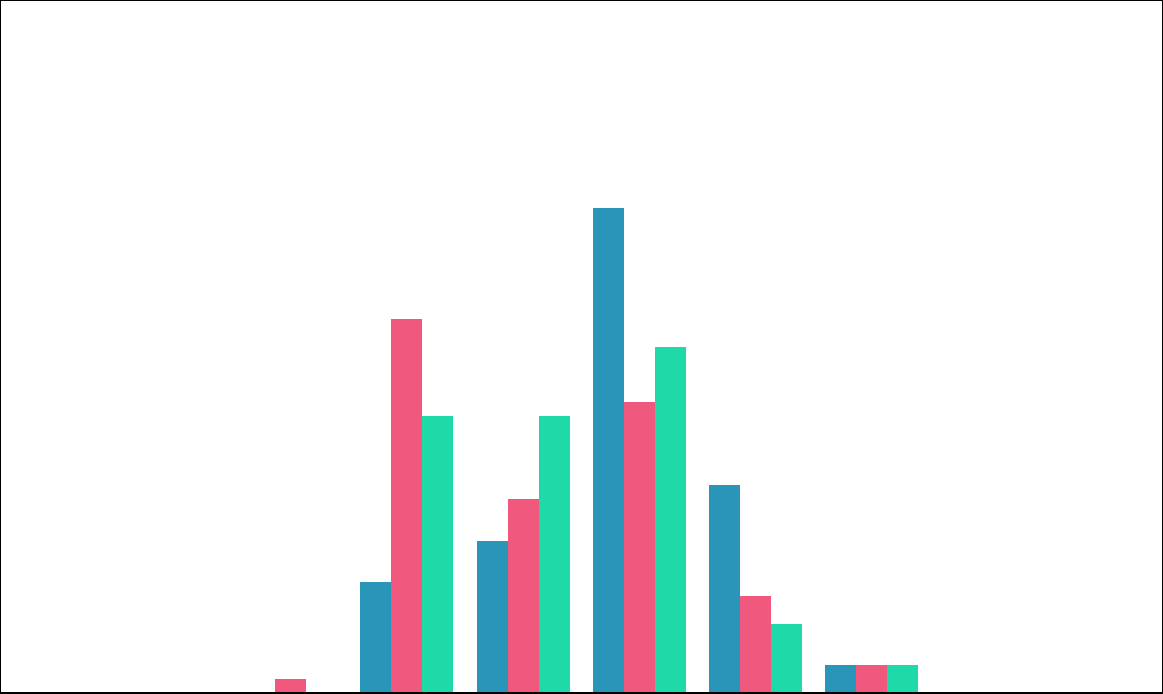}
        \end{minipage}
        &
        \begin{minipage}{.095 \textwidth}
            \includegraphics[width=\linewidth]{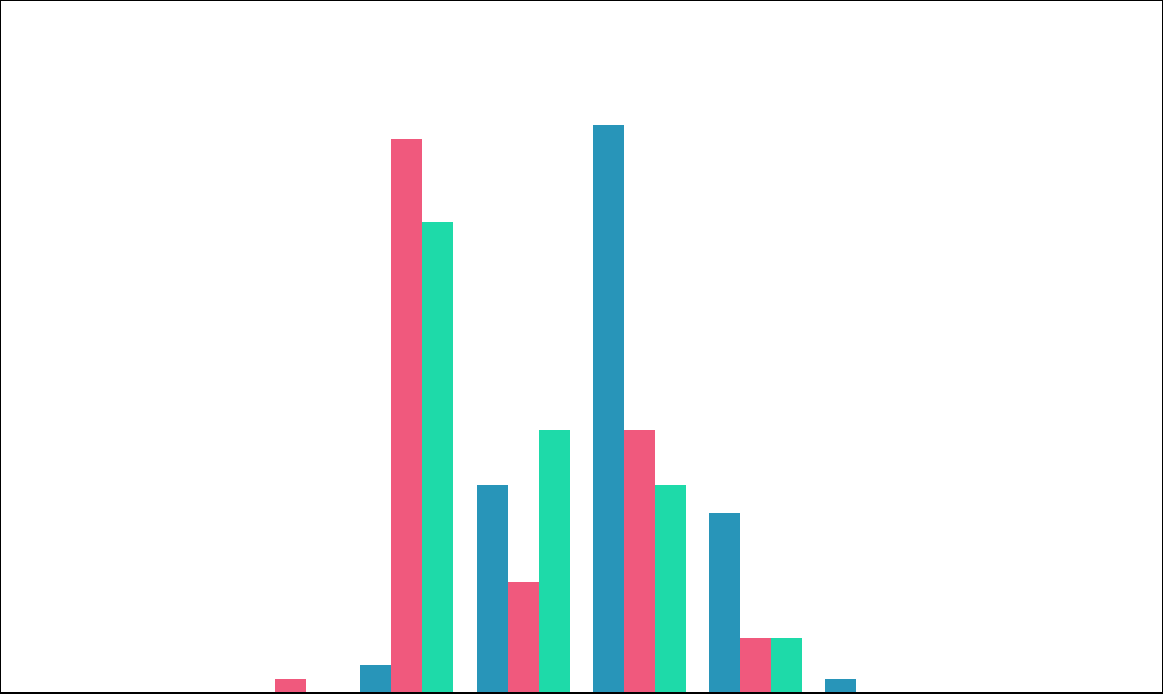}
        \end{minipage}
        \\          
    \end{tabular}
    \Caption{Visualization of all participants, conditions and scenes of the user study \Cref{sec:results:study}.
    }{%
    X-axis indicates time (0-1000ms). Y-axis indicates density. Each color of the stacked bars indicates each condition: blue/red/green represents $\conditionEvalStudyVergent:\vergentAmp= 0^\circ$ / $\conditionEvalStudyCombinedShort:\vergentAmp= 7^\circ$ / $\conditionEvalStudyCombinedLong:\vergentAmp= 10.5^\circ$. The inset numbers are the corresponding K.S. test results for each user across all conditions and scenes. Note that the  discrepancy between eye travel distance ($\conditionEvalStudyVergent<\conditionEvalStudyCombinedShort<\conditionEvalStudyCombinedLong$) and landing times ($\conditionEvalStudyCombinedShort<\conditionEvalStudyCombinedLong<\conditionEvalStudyVergent$) share statistical significance across individuals.
    }
    \label{fig:appendix:eval}
\end{figure}
