# Supplementary material for: The Shortest Route Is Not Always the Fastest: Probability-Modeled Stereoscopic Eye Movement Completion Time in VR
Source: arXiv:2309.15183 source file (2023-10-03)
Supplement: Supplementary file 3 [file fig_supp_results_errorbars.tex]

\begin{figure}[h]
    \centering
    \subfloat[saccade]{
        \vphantom{\includegraphics[width=0.290\linewidth,valign=t]{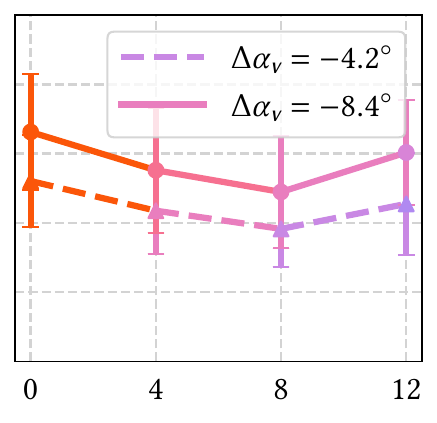}}
        \includegraphics[width=0.330\linewidth,valign=t]{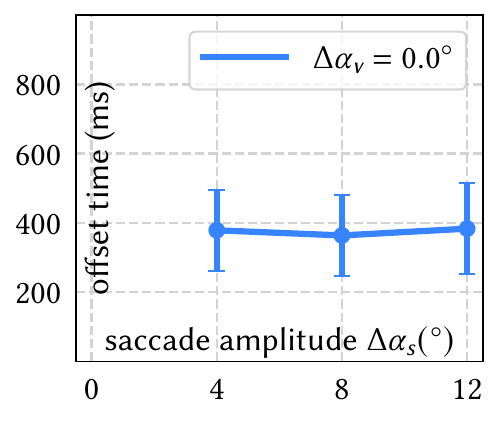} \label{fig:supp:results:saccade}
    }%subfloat
    \subfloat[divergent]{
        \includegraphics[width=0.290\linewidth,valign=t]{figures/pilot_data_aggregate_divergent_errorbar.pdf}
        \label{fig:supp:results:divergent}
    }%subfloat
    \subfloat[convergent]{
        \includegraphics[width=0.290\linewidth,valign=t]{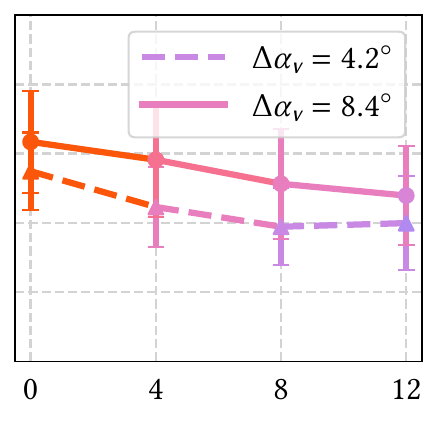}
        \label{fig:supp:results:convergent}
    }%subfloat
    \Caption{
        Aggregated mean offset time of studied conditions across all participants with error bars.
    }{%
        This is a version of \Cref{fig:pilot:summary} with std error bars as a more detailed visualization.
        See \Cref{fig:pilot:summary} for further details.
    }
\label{fig:supp:results}
\end{figure}
