# Supplementary material for: The Shortest Route Is Not Always the Fastest: Probability-Modeled Stereoscopic Eye Movement Completion Time in VR
Source: arXiv:2309.15183 source file (2023-10-03)
Supplement: Supplementary file 4 [file fig_supp_study_conditions.tex]

\begin{figure}[h]
    \centering
    \subfloat[divergent]{
        \includegraphics[width=0.45\linewidth]{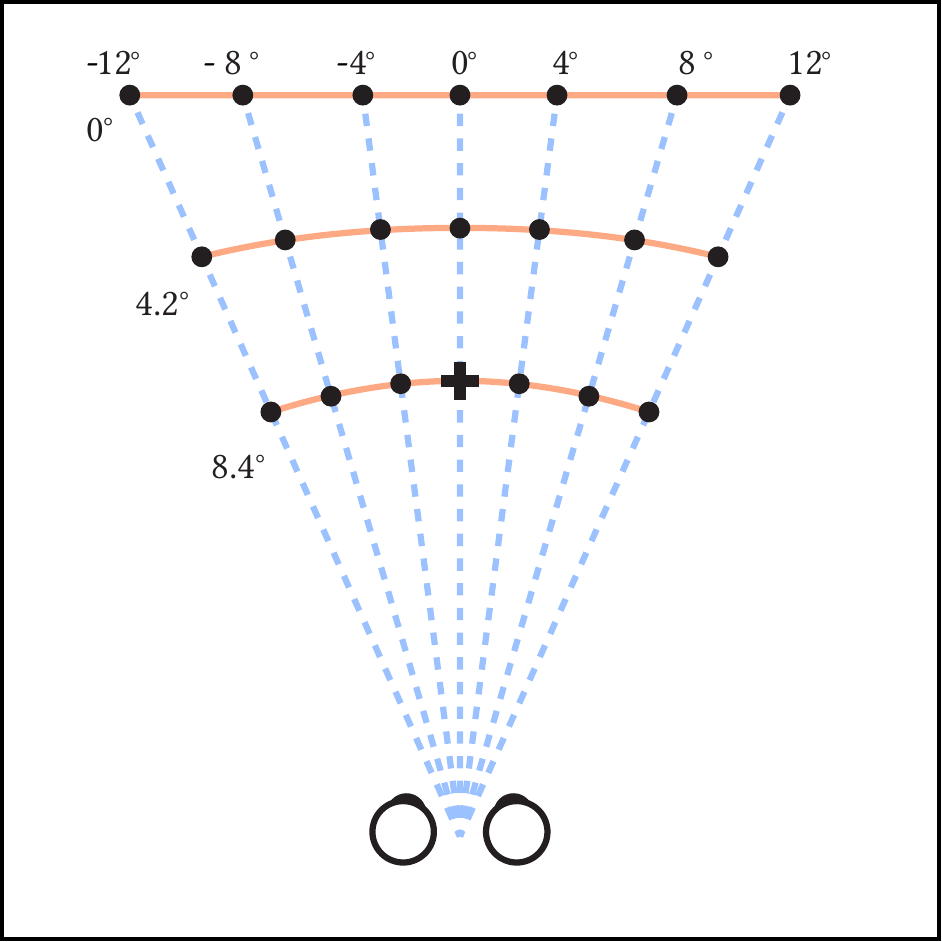}
        \label{fig:supp:study:conditions:divergent}
    }%subfloat
    \hfill
    \subfloat[convergent]{
        \includegraphics[width=0.45\linewidth]{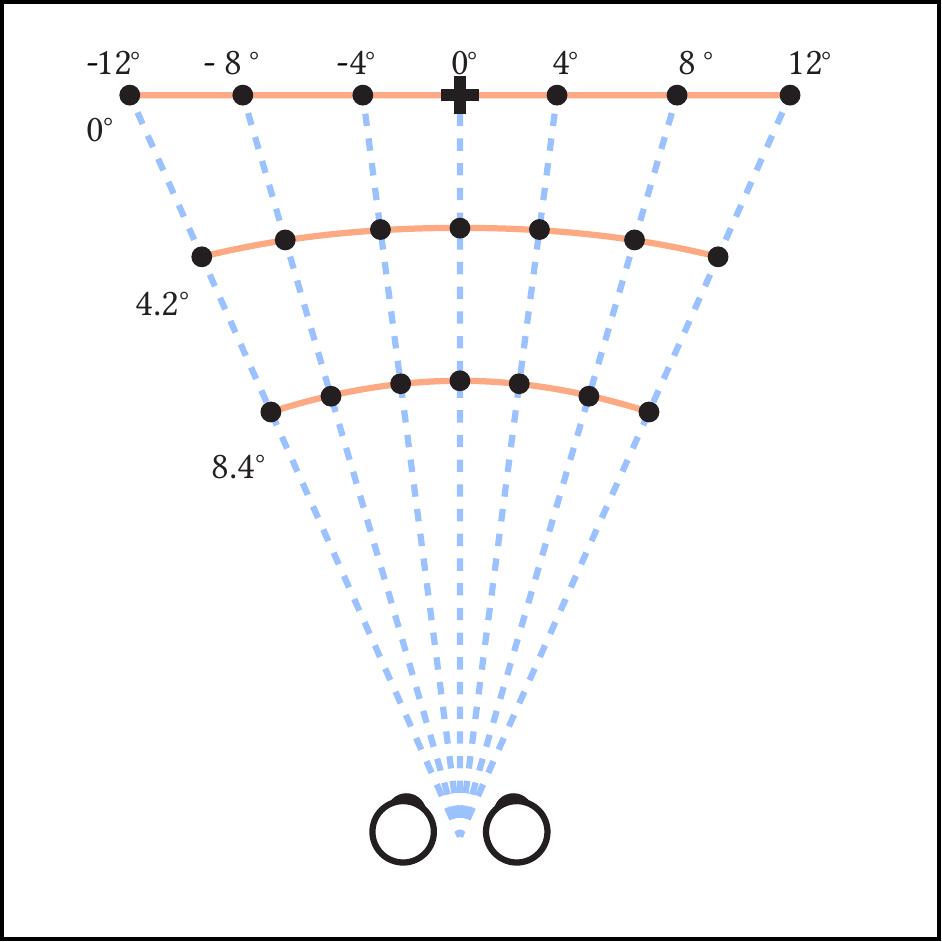}
        \label{fig:supp:study:conditions:convergent}
    }%subfloat
    \Caption{
       Study conditions.
    }{
        All visualized conditions originate at a $+$ sign (near for divergent, far for convergent conditions), and target $\cdot$ signs.
        Leftward and rightward saccades are treated as equivalent in data analysis, but there are equal number of leftward and rightward conditions implemented.
    }
\label{fig:supp:study:conditions}
\end{figure}
