# Supplementary material for: The Shortest Route Is Not Always the Fastest: Probability-Modeled Stereoscopic Eye Movement Completion Time in VR
Source: arXiv:2309.15183 source file (2023-10-03)
Supplement: Supplementary file 5 [file sec_supp.tex]

% Uncomment next line to make a one-column supplement
% \onecolumn
\section{Display Specifications}
\label{tab:pilot:hmd}
\input{tab_pilot_hmd}

\section{Psychophysical Study Conditions}
\label{sec:supp:pilot:conditions}

\paragraph{Calibration of maximum vergence amplitudes}

The closest depth at which majority of user study participants could fuse a stereo image in VR was approximately $\minDepth = 0.4\ \text{m}$.
Depth, $\depth$, and vergence angle coordinates, $\vergentAng$, have an inversely proportional relationship,
%
\begin{align}
\vergentAng = \arctan\left(\frac{\ipd}{2 \depth}\right),
\label{eqn:vergence-ang-derivation}
\end{align}
%
which varies from person to person depending on their IPD, $\ipd$.
This relationship, and the fact that there are no negative vergence angle coordinates, effectively limits the range of vergence gaze movement amplitudes, $\vergentAmp$, a user study participant can make.
Crucially, since the IPD, $\ipd$, of participants varied, and we couldn't foresee the IPDs of all future user study participants, we could not determine the maximum vergence angle coordinate, $\vergentAng^{max}$, by applying \Cref{eqn:vergence-ang-derivation} naively.
Therefore, to ensure consistency across different participants, we selected the most conservative value of maximum vergence angle coordinates by minimizing \Cref{eqn:vergence-ang-derivation} under the constraints of $\depth > \minDepth = 0.4\ \text{m}$, and $\ipd > \ipd^\textit{min} = 59\ \text{mm}$ --- the minimum IPD supported by the HMD.
Then, applying these edge conditions to \Cref{eqn:vergence-ang-derivation}, we get our maximum vergence angle coordinate of $\vergentAng^\textit{max} = 8.4^\circ$.

\input{fig_supp_study_conditions}

\paragraph{Implementation of Study Conditions}
We construct three isovergence circles for each  $\vergentAng^\textit{init}+\vergentAmp$, starting with the smallest.
As established earlier, this circle must be at least $\minDepth$ away from the observer.
Therefore we pick the first isovergence circle to be $\depth^{(0)} = \minDepth$ away, which corresponds to a vergence angle coordinate equal to
%
\begin{align}
\vergentAng^{(0)} = \arctan\left(\frac{\ipd}{2\depth^{(0)}}\right).
\end{align}
%
The following circles are constructed by adding the $\vergentAmp$ to $\vergentAng^{(0)}$:
%
\begin{align}
\vergentAng^{(i)} = \vergentAng^{(0)} + \vergentAmp^{(i-1)},
\text{ for } i \in \{1, 2\},
\end{align}
%
where $\vergentAmp^{(i-1)}$ is the $i-1$th condition among vergence conditions.

Equipped with the isovergence circles with angles $\{\vergentAng^{(i)}\}$ for $i \in \{0, 1, 2\}$, we can select the initial fixation point for all divergent and convergent gaze motions to be at coordinates
%
\begin{align}
\begin{aligned}
(\vergentAng^\textit{init, div}, \saccadeAng^\textit{init, div})
= (\vergentAng^{(0)}, 0^\circ)\\
(\vergentAng^\textit{init, conv}, \saccadeAng^\textit{init, conv})
= (\vergentAng^{(2)}, 0^\circ),
\end{aligned}
\end{align}
%
respectively.
Originating from a given fixation point, the rest of the condition locations are found as
%
\begin{align}
(\vergentAng, \saccadeAng) = (\vergentAng^\textit{init} + \vergentAmp, \saccadeAng^{init} + \saccadeAmp),
\end{align}
%
where $\vergentAmp$ and $\saccadeAmp$ correspond to the specific experimental condition of interest.
The resulting grid of conditions are visualized in \Cref{fig:supp:study:conditions}.

\section{Experiment Results}
\label{sec:supp:results}
\input{fig_supp_results_errorbars}

\clearpage

\section{Ablation Study Histograms}
\label{sec:supp:ablation}
\input{fig_supp_ablation_histograms}
\newpage

\section{Full Statistical Visualization of User Study}
\label{sec:supp:study:fullStats}

\input{fig_supp_eval_tile.tex}
